# Supplementary material for: Exploring the Statically Screened $G3W2$ Correction to the $GW$ Self-Energy: Charged Excitations and Total Energies of Finite Systems
Source: arXiv:2110.04105 ancillary file (2022-03-17)
Supplement: Supplementary file 1 [file SI.pdf]

# Supporting information for: Exploring the Statically Screened $G3W2$ Correction to the $GW$ Self-Energy: Charged Excitations and Total Energies of Finite Systems

Arno Förster* and Lucas Visscher
*Theoretical Chemistry, Vrije Universiteit, De Boelelaan 1083, NL-1081 HV, Amsterdam, The Netherlands*
(Dated: January 25, 2022)

## CONTENTS

I. Total Correlation Energies 3

II. Charged Excitations for 24 Organic Acceptor molecules 4
A. Individual QP energies and technical parameters 4
1. qsGW(+$G3W2$)/TZ3P 4
2. qsGW(+$G3W2$)/QZ6P 5
3. $G_0W_0$(+$G3W2$)@LRC-$\omega$PBEh/TZ3P 6
4. $G_0W_0$(+$G3W2$)@LRC-$\omega$PBEh/QZ6P 7
5. $G_0W_0$(+$G3W2$)@$\omega$B97-X/TZ3P 8
6. $G_0W_0$(+$G3W2$)@$\omega$B97-X/QZ6P 9
7. $G_0W_0$(+$G3W2$)@PBE0/TZ3P 10
8. $G_0W_0$(+$G3W2$)@PBE0/QZ6P 11
9. $G_0W_0$(+$G3W2$)@PBE/TZ3P 12
10. $G_0W_0$(+$G3W2$)@PBE/QZ6P 13
B. Basis set limit extrapolated QP energies and comparison to CCSD(T) reference values 14
1. qsGW - ionization potentials 14
2. LRC-$\omega$PBEh - ionization potentials 15
3. $\omega$B97-X - ionization potentials 16
4. PBE0 - ionization potentials 17
5. PBE - ionization potentials 18
6. qsGW - electron affinities 19
7. LRC-$\omega$PBEh - electron affinities 20
8. $\omega$B97-X - electron affinities 21
9. PBE0 - electron affinities 22
10. PBE - electron affinities 23
11. qsGW - fundamental gaps 24
12. LRC-$\omega$PBEh - fundamental gaps 25
13. $\omega$B97-X - fundamental gaps 26
14. PBE0 - fundamental gaps 27
15. PBE - fundamental gaps 28

III. Ionization potentials for 40 small molecules (gw40) 29
A. Individual QP energies and technical parameters 29
1. qsGW(+$G3W2$)/TZ3P 29
2. qsGW(+$G3W2$)/QZ6P 30
3. $G_0W_0$(+$G3W2$)@LRC-$\omega$PBEh/TZ3P 31
4. $G_0W_0$(+$G3W2$)@LRC-$\omega$PBEh/QZ6P 32
5. $G_0W_0$(+$G3W2$)@$\omega$B97-X/TZ3P 33
6. $G_0W_0$(+$G3W2$)@$\omega$B97-X/QZ6P 34
B. Basis set limit extrapolated QP energies and comparison to EOM-CCSDT reference values 35
1. qsGW - ionization potentials 35
2. LRC-$\omega$PBEh - ionization potentials 36
3. $\omega$B97-X - ionization potentials 37

References 38

The supporting information contains

- All values calculated in this work
  - Total (in PDF and csv format) and relative energies (csv format)
  - QP energies (in PDF and in csv format)
- Details on basis sets used. The augmented basis sets used for the calculation of the total correlation energies are available here and are based on the basis sets described (and available online).[1]

All numbers shown here can be reproduced from the numbers provided in the .csv files. References to the data which has not been generated for this work can be found in the main paper.

## I. TOTAL CORRELATION ENERGIES

| | aug-TZ3P | | aug-QZ6P | | extrapolated | | reference |
|---|---|---|---|---|---|---|---|
| Atom | RPA+SOSSX | RPA | RPA+SOSSX | RPA | RPA+SOSSX | RPA | ref. |
| Be2+ | −0.052 | −0.079 | −0.061 | −0.084 | 0.067 | 0.087 | 0.044 |
| Li+ | −0.055 | −0.078 | −0.059 | −0.083 | 0.062 | 0.087 | 0.054 |
| He | −0.060 | −0.081 | −0.061 | −0.083 | 0.061 | 0.084 | 0.042 |
| B | −0.116 | −0.177 | −0.045 | −0.181 | −0.007 | 0.185 | 0.111 |
| Be | −0.102 | −0.151 | −0.106 | −0.157 | 0.108 | 0.162 | 0.094 |
| Mg2+ | −0.302 | −0.389 | −0.362 | −0.470 | 0.406 | 0.528 | 0.390 |
| Na+ | −0.304 | −0.389 | −0.366 | −0.475 | 0.410 | 0.538 | 0.389 |
| Ne | −0.426 | −0.523 | −0.424 | −0.558 | 0.423 | 0.583 | 0.390 |
| Si2+ | −0.350 | −0.442 | −0.457 | −0.589 | 0.535 | 0.695 | 0.463 |
| Mg | −0.364 | −0.455 | −0.420 | −0.538 | 0.461 | 0.598 | 0.438 |
| Ca2+ | −0.499 | −0.625 | −0.695 | −0.896 | 0.838 | 1.093 | 0.754 |
| K+ | −0.525 | −0.679 | −0.671 | −0.854 | 0.778 | 0.982 | 0.739 |
| Ar | −0.520 | −0.668 | −0.667 | −0.851 | 0.774 | 0.985 | 0.722 |
| Ca | −0.551 | −0.689 | −0.749 | −0.964 | 0.894 | 1.164 | 0.827 |
| Zn | −1.143 | −1.352 | −1.457 | −1.714 | 1.686 | 1.978 | 1.621 |
| Kr | −0.908 | −1.115 | −1.449 | −1.771 | 1.844 | 2.250 | 1.850 |

TABLE I. Total correlation energies at the RPA+SOSSX@OEP and RPA@OEP levels of theory using the augmented TZ3P, augmented QZ6P basis set as well as extrapolated values and reference values.[2,3]

# II. CHARGED EXCITATIONS FOR 24 ORGANIC ACCEPTOR MOLECULES

## A. Individual QP energies and technical parameters

### 1. qsGW(+G3W2)/TZ3P

| | GW | | GW + G3W2 | | | | |
|---|---|---|---|---|---|---|---|
| molecule | IP | EA | IP | EA | $N_{bas}$ | $N_{freq}$ | $N_{time}$ |
| Anthracene | 7.31 | 0.14 | 7.22 | −0.04 | 555 | 15 | 15 |
| Acridine | 7.80 | 0.49 | 7.74 | 0.32 | 543 | 16 | 16 |
| phenazine | 8.21 | 0.92 | 8.17 | 0.77 | 530 | 15 | 15 |
| Azulene | 7.25 | 0.35 | 7.21 | 0.17 | 408 | 15 | 15 |
| Benzoquinone | 10.55 | 1.36 | 10.65 | 1.27 | 298 | 15 | 15 |
| Naphthalenedione | 9.72 | 1.26 | 9.79 | 1.14 | 444 | 16 | 16 |
| Dichlone | 9.77 | 1.67 | 9.81 | 1.55 | 496 | 17 | 17 |
| tetrafluorobenzoquinone | 11.32 | 2.19 | 11.38 | 2.10 | 369 | 17 | 17 |
| tetrachlorobenzoquinone | 10.13 | 2.21 | 10.17 | 2.11 | 401 | 17 | 17 |
| Nitrobenzene | 10.04 | 0.37 | 10.07 | 0.23 | 341 | 15 | 15 |
| tetrafluorobenzenedicarbonitrile | 10.68 | 1.51 | 10.76 | 1.36 | 429 | 15 | 15 |
| Dinitrobenzonitrile | 11.04 | 1.63 | 11.09 | 1.50 | 468 | 15 | 15 |
| Nitrobenzonitrile | 10.47 | 1.19 | 10.51 | 1.06 | 389 | 17 | 17 |
| Benzonitrile | 9.72 | −0.45 | 9.71 | −0.63 | 310 | 14 | 14 |
| Fumaronitrile | 11.27 | 0.72 | 11.23 | 0.60 | 211 | 15 | 15 |
| mDCNB | 10.22 | 0.39 | 10.22 | 0.22 | 358 | 15 | 15 |
| TCNE | 11.77 | 2.83 | 11.76 | 2.73 | 309 | 14 | 14 |
| TCNQ | 9.38 | 3.18 | 9.30 | 3.10 | 543 | 15 | 15 |
| Maleicanhydride | 11.56 | 0.81 | 11.71 | 0.69 | 241 | 15 | 15 |
| Phthalimide | 9.94 | 0.43 | 9.98 | 0.28 | 401 | 15 | 15 |
| phthalicanhydride | 10.37 | 0.70 | 10.42 | 0.54 | 388 | 17 | 17 |
| tetrachloro-isobenzofuranedione | 9.87 | 1.43 | 9.92 | 1.27 | 491 | 17 | 17 |
| NDCA | 8.98 | 1.10 | 8.96 | 0.95 | 534 | 16 | 16 |
| bodipy | 7.92 | 1.41 | 7.86 | 1.28 | 516 | 15 | 15 |

TABLE II. Ionization potentials and electron affinities at the qsGW(+$G3W2$)/TZ3P level of theory (in eV) as well as total number of molecular orbitals and size of imaginary time and imaginary frequency grids for the acc24 test set.

### 2. qsGW(+G3W2)/QZ6P

| molecule | GW IP | GW EA | GW + G3W2 IP | GW + G3W2 EA | $N_{bas}$ | $N_{freq}$ | $N_{time}$ |
|---|---|---|---|---|---|---|---|
| Anthracene | 7.41 | 0.33 | 7.29 | 0.11 | 965 | 17 | 17 |
| Acridine | 7.89 | 0.66 | 7.80 | 0.46 | 946 | 18 | 18 |
| phenazine | 8.35 | 1.09 | 8.27 | 0.90 | 929 | 18 | 18 |
| Azulene | 7.42 | 0.51 | 7.34 | 0.29 | 713 | 17 | 17 |
| Benzoquinone | 10.61 | 1.48 | 10.68 | 1.34 | 515 | 18 | 18 |
| Naphthalenedione | 9.82 | 1.40 | 9.85 | 1.25 | 768 | 18 | 18 |
| Dichlone | 9.85 | 1.79 | 9.84 | 1.63 | 866 | 24 | 24 |
| tetrafluorobenzoquinone | 11.24 | 2.29 | 11.25 | 2.16 | 644 | 19 | 19 |
| tetrachlorobenzoquinone | 10.20 | 2.32 | 10.19 | 2.18 | 715 | 23 | 23 |
| Nitrobenzene | 10.11 | 0.53 | 10.11 | 0.35 | 595 | 18 | 18 |
| tetrafluorobenzenedicarbonitrile | 10.78 | 1.66 | 10.81 | 1.47 | 757 | 18 | 18 |
| Dinitrobenzonitrile | 11.08 | 1.76 | 11.09 | 1.59 | 813 | 18 | 18 |
| Nitrobenzonitrile | 10.57 | 1.31 | 10.57 | 1.15 | 678 | 18 | 18 |
| Benzonitrile | 9.80 | −0.26 | 9.75 | −0.47 | 542 | 17 | 17 |
| Fumaronitrile | 11.35 | 0.87 | 11.28 | 0.71 | 400 | 17 | 17 |
| mDCNB | 10.31 | 0.57 | 10.27 | 0.36 | 627 | 17 | 17 |
| TCNE | 11.95 | 3.02 | 11.91 | 2.88 | 539 | 17 | 17 |
| TCNQ | 9.47 | 3.31 | 9.36 | 3.20 | 940 | 18 | 18 |
| Maleicanhydride | 11.62 | 0.92 | 11.74 | 0.76 | 415 | 18 | 18 |
| Phthalimide | 10.03 | 0.57 | 10.03 | 0.38 | 695 | 18 | 18 |
| phthalicanhydride | 10.45 | 0.82 | 10.46 | 0.62 | 666 | 18 | 18 |
| tetrachloro-isobenzofuranedione | 9.93 | 1.55 | 9.93 | 1.35 | 862 | 24 | 24 |
| NDCA | 9.04 | 1.23 | 8.99 | 1.04 | 916 | 18 | 18 |
| bodipy | 8.04 | 1.55 | 7.95 | 1.37 | 913 | 18 | 18 |

TABLE III. Ionization potentials and electron affinities at the qsGW(+$G3W2$)/QZ6P level of theory (in eV) as well as total number of molecular orbitals and size of imaginary time and imaginary frequency grids for the acc24 test set.

### 3. $G_0W_0$(+$G3W2$)@LRC-$\omega$PBEh/TZ3P

| | GW | | $GW + G3W2$ | | | | |
|---|---|---|---|---|---|---|---|
| molecule | IP | EA | IP | EA | $N_{bas}$ | $N_{freq}$ | $N_{time}$ |
| Anthracene | 7.27 | 0.19 | 7.18 | 0.00 | 555 | 16 | 16 |
| Acridine | 7.79 | 0.54 | 7.73 | 0.37 | 543 | 16 | 16 |
| phenazine | 8.22 | 0.97 | 8.19 | 0.81 | 530 | 16 | 16 |
| Azulene | 7.28 | 0.39 | 7.23 | 0.19 | 408 | 16 | 16 |
| Benzoquinone | 10.31 | 1.39 | 10.42 | 1.28 | 298 | 17 | 17 |
| Naphthalenedione | 9.96 | 1.27 | 10.09 | 1.15 | 444 | 16 | 16 |
| Dichlone | 9.69 | 1.70 | 9.74 | 1.57 | 496 | 18 | 18 |
| tetrafluorobenzoquinone | 10.93 | 2.15 | 11.00 | 2.05 | 369 | 17 | 17 |
| tetrachlorobenzoquinone | 10.00 | 2.25 | 10.05 | 2.14 | 401 | 18 | 18 |
| Nitrobenzene | 10.00 | 0.36 | 10.02 | 0.21 | 341 | 17 | 17 |
| tetrafluorobenzenedicarbonitrile | 10.54 | 1.51 | 10.63 | 1.36 | 429 | 16 | 16 |
| Dinitrobenzonitrile | 11.03 | 1.60 | 11.08 | 1.46 | 468 | 17 | 17 |
| Nitrobenzonitrile | 10.48 | 1.18 | 10.51 | 1.05 | 389 | 18 | 18 |
| Benzonitrile | 9.76 | −0.37 | 9.75 | −0.56 | 310 | 15 | 15 |
| Fumaronitrile | 11.21 | 0.84 | 11.18 | 0.70 | 211 | 15 | 15 |
| mDCNB | 10.26 | 0.47 | 10.26 | 0.30 | 358 | 16 | 16 |
| TCNE | 11.71 | 2.96 | 11.73 | 2.86 | 309 | 16 | 16 |
| TCNQ | 9.34 | 3.30 | 9.28 | 3.22 | 543 | 17 | 17 |
| Maleicanhydride | 11.31 | 0.82 | 11.47 | 0.69 | 241 | 18 | 18 |
| Phthalimide | 10.32 | 0.43 | 10.48 | 0.27 | 401 | 17 | 17 |
| phthalicanhydride | 10.34 | 0.69 | 10.38 | 0.53 | 388 | 17 | 17 |
| tetrachloro-isobenzofuranedione | 9.83 | 1.45 | 9.89 | 1.28 | 491 | 17 | 17 |
| NDCA | 8.92 | 1.12 | 8.90 | 0.96 | 534 | 18 | 18 |
| bodipy | 7.95 | 1.45 | 7.88 | 1.31 | 516 | 17 | 17 |

TABLE IV. Ionization potentials and electron affinities at the LRC-$\omega$PBEh(+$G3W2$)/TZ3P level of theory (in eV) as well as total number of molecular orbitals and size of imaginary time and imaginary frequency grids for the acc24 test set.

#### 4. $G_0W_0$(+$G3W2$)@LRC-$\omega$PBEh/QZ6P

| | $GW$ | | $GW+G3W2$ | | | | |
|---|---|---|---|---|---|---|---|
| molecule | IP | EA | IP | EA | $N_{bas}$ | $N_{freq}$ | $N_{time}$ |
| Anthracene | 7.42 | 0.40 | 7.26 | 0.12 | 965 | 18 | 18 |
| Acridine | 7.92 | 0.74 | 7.79 | 0.48 | 946 | 18 | 18 |
| phenazine | 8.36 | 1.16 | 8.26 | 0.92 | 929 | 18 | 18 |
| Azulene | 7.44 | 0.58 | 7.32 | 0.30 | 713 | 18 | 18 |
| Benzoquinone | 10.42 | 1.54 | 10.49 | 1.35 | 515 | 18 | 18 |
| Naphthalenedione | 10.06 | 1.46 | 10.17 | 1.25 | 768 | 19 | 19 |
| Dichlone | 9.86 | 1.88 | 9.84 | 1.68 | 866 | 24 | 24 |
| tetrafluorobenzoquinone | 11.06 | 2.32 | 11.06 | 2.14 | 644 | 19 | 19 |
| tetrachlorobenzoquinone | 10.16 | 2.43 | 10.14 | 2.24 | 715 | 24 | 24 |
| Nitrobenzene | 10.11 | 0.56 | 10.08 | 0.33 | 595 | 19 | 19 |
| tetrafluorobenzenedicarbonitrile | 10.67 | 1.71 | 10.69 | 1.48 | 757 | 19 | 19 |
| Dinitrobenzonitrile | 11.15 | 1.78 | 11.15 | 1.56 | 813 | 18 | 18 |
| Nitrobenzonitrile | 10.62 | 1.38 | 10.60 | 1.16 | 678 | 18 | 18 |
| Benzonitrile | 9.89 | −0.16 | 9.80 | −0.43 | 542 | 17 | 17 |
| Fumaronitrile | 11.36 | 1.01 | 11.28 | 0.80 | 400 | 17 | 17 |
| mDCNB | 10.43 | 0.68 | 10.36 | 0.42 | 627 | 18 | 18 |
| TCNE | 11.84 | 3.13 | 11.82 | 2.96 | 539 | 18 | 18 |
| TCNQ | 9.49 | 3.47 | 9.36 | 3.30 | 940 | 18 | 18 |
| Maleicanhydride | 11.41 | 0.99 | 11.56 | 0.78 | 415 | 19 | 19 |
| Phthalimide | 10.39 | 0.63 | 10.54 | 0.39 | 695 | 19 | 19 |
| phthalicanhydride | 10.47 | 0.88 | 10.45 | 0.64 | 666 | 18 | 18 |
| tetrachloro-isobenzofuranedione | 9.99 | 1.64 | 9.98 | 1.40 | 862 | 24 | 24 |
| NDCA | 9.06 | 1.30 | 8.97 | 1.05 | 916 | 18 | 18 |
| bodipy | 8.10 | 1.62 | 7.97 | 1.38 | 913 | 20 | 20 |

TABLE V. Ionization potentials and electron affinities at the LRC-$\omega$PBEh(+$G3W2$)/QZ6P level of theory (in eV) as well as total number of molecular orbitals and size of imaginary time and imaginary frequency grids for the acc24 test set.

### 5. $G_0W_0(+G3W2)$@$\omega B97$-$X/TZ3P$

| | $GW$ | | $GW+G3W2$ | | | | |
|---|---|---|---|---|---|---|---|
| molecule | IP | EA | IP | EA | $N_{bas}$ | $N_{freq}$ | $N_{time}$ |
| Anthracene | 7.36 | 0.17 | 7.27 | −0.02 | 555 | 16 | 16 |
| Acridine | 7.86 | 0.52 | 7.80 | 0.35 | 543 | 16 | 16 |
| phenazine | 8.31 | 0.96 | 8.27 | 0.80 | 530 | 16 | 16 |
| Azulene | 7.35 | 0.40 | 7.30 | 0.20 | 408 | 16 | 16 |
| Benzoquinone | 10.46 | 1.37 | 10.58 | 1.27 | 298 | 18 | 18 |
| Naphthalenedione | 9.78 | 1.26 | 9.85 | 1.14 | 444 | 17 | 17 |
| Dichlone | 9.80 | 1.69 | 9.85 | 1.57 | 496 | 18 | 18 |
| tetrafluorobenzoquinone | 11.06 | 2.14 | 11.13 | 2.05 | 369 | 18 | 18 |
| tetrachlorobenzoquinone | 10.14 | 2.25 | 10.18 | 2.15 | 401 | 18 | 18 |
| Nitrobenzene | 10.08 | 0.36 | 10.12 | 0.21 | 341 | 15 | 15 |
| tetrafluorobenzenedicarbonitrile | 10.66 | 1.51 | 10.74 | 1.36 | 429 | 16 | 16 |
| Dinitrobenzonitrile | 11.14 | 1.61 | 11.19 | 1.48 | 468 | 18 | 18 |
| Nitrobenzonitrile | 10.60 | 1.18 | 10.63 | 1.05 | 389 | 16 | 16 |
| Benzonitrile | 9.81 | −0.39 | 9.80 | −0.58 | 310 | 16 | 16 |
| Fumaronitrile | 11.31 | 0.82 | 11.28 | 0.69 | 211 | 15 | 15 |
| mDCNB | 10.36 | 0.47 | 10.36 | 0.29 | 358 | 15 | 15 |
| TCNE | 11.84 | 2.95 | 11.85 | 2.85 | 309 | 16 | 16 |
| TCNQ | 9.48 | 3.29 | 9.40 | 3.22 | 543 | 17 | 17 |
| Maleicanhydride | 11.42 | 0.82 | 11.59 | 0.69 | 241 | 16 | 16 |
| Phthalimide | 9.98 | 0.43 | 10.02 | 0.27 | 401 | 18 | 18 |
| phthalicanhydride | 10.43 | 0.69 | 10.48 | 0.53 | 388 | 16 | 16 |
| tetrachloro-isobenzofuranedione | 9.95 | 1.47 | 10.01 | 1.31 | 491 | 18 | 18 |
| NDCA | 9.01 | 1.10 | 8.99 | 0.94 | 534 | 17 | 17 |
| bodipy | 8.03 | 1.45 | 7.96 | 1.31 | 516 | 16 | 16 |

TABLE VI. Ionization potentials and electron affinities at the $\omega$B97-X($+G3W2$)/TZ3P level of theory (in eV) as well as total number of molecular orbitals and size of imaginary time and imaginary frequency grids for the acc24 test set.

### 6. $G_0W_0(+G3W2)$@$\omega B97$-X/QZ6P

| | $GW$ | | $GW+G3W2$ | | | | |
|---|---|---|---|---|---|---|---|
| molecule | IP | EA | IP | EA | $N_{bas}$ | $N_{freq}$ | $N_{time}$ |
| Anthracene | 7.50 | 0.40 | 7.34 | 0.13 | 965 | 17 | 17 |
| Acridine | 8.02 | 0.74 | 7.89 | 0.49 | 946 | 17 | 17 |
| phenazine | 8.46 | 1.17 | 8.35 | 0.93 | 929 | 17 | 17 |
| Azulene | 7.51 | 0.61 | 7.40 | 0.33 | 713 | 18 | 18 |
| Benzoquinone | 10.59 | 1.54 | 10.67 | 1.37 | 515 | 18 | 18 |
| Naphthalenedione | 9.94 | 1.45 | 9.94 | 1.25 | 768 | 19 | 19 |
| Dichlone | 9.98 | 1.89 | 9.96 | 1.69 | 866 | 24 | 24 |
| tetrafluorobenzoquinone | 11.21 | 2.31 | 11.21 | 2.14 | 644 | 18 | 18 |
| tetrachlorobenzoquinone | 10.30 | 2.43 | 10.29 | 2.26 | 715 | 24 | 24 |
| Nitrobenzene | 10.17 | 0.57 | 10.14 | 0.35 | 595 | 18 | 18 |
| tetrafluorobenzenedicarbonitrile | 10.79 | 1.71 | 10.82 | 1.49 | 757 | 19 | 19 |
| Dinitrobenzonitrile | 11.28 | 1.81 | 11.28 | 1.60 | 813 | 18 | 18 |
| Nitrobenzonitrile | 10.71 | 1.38 | 10.68 | 1.17 | 678 | 19 | 19 |
| Benzonitrile | 10.02 | −0.17 | 9.94 | −0.43 | 542 | 17 | 17 |
| Fumaronitrile | 11.45 | 1.00 | 11.37 | 0.80 | 400 | 18 | 18 |
| mDCNB | 10.54 | 0.68 | 10.48 | 0.43 | 627 | 18 | 18 |
| TCNE | 11.99 | 3.12 | 11.95 | 2.96 | 539 | 17 | 17 |
| TCNQ | 9.63 | 3.46 | 9.49 | 3.31 | 940 | 19 | 19 |
| Maleicanhydride | 11.56 | 0.98 | 11.72 | 0.79 | 415 | 18 | 18 |
| Phthalimide | 10.14 | 0.64 | 10.12 | 0.40 | 695 | 18 | 18 |
| phthalicanhydride | 10.56 | 0.89 | 10.55 | 0.65 | 666 | 19 | 19 |
| tetrachloro-isobenzofuranedione | 10.12 | 1.67 | 10.11 | 1.43 | 862 | 24 | 24 |
| NDCA | 9.16 | 1.30 | 9.08 | 1.06 | 916 | 18 | 18 |
| bodipy | 8.19 | 1.64 | 8.05 | 1.40 | 913 | 20 | 20 |

TABLE VII. Ionization potentials and electron affinities at the $\omega$B97-X(+$G3W2$)/QZ6P level of theory (in eV) as well as total number of molecular orbitals and size of imaginary time and imaginary frequency grids for the acc24 test set.

### 7. $G_0W_0$(+$G3W2$)@PBE0/TZ3P

| | $GW$ | | $GW+G3W2$ | | | | |
|---|---|---|---|---|---|---|---|
| molecule | IP | EA | IP | EA | $N_{bas}$ | $N_{freq}$ | $N_{time}$ |
| Anthracene | 7.04 | 0.37 | 6.95 | 0.17 | 555 | 16 | 16 |
| Acridine | 7.52 | 0.70 | 7.46 | 0.51 | 543 | 17 | 17 |
| phenazine | 7.94 | 1.10 | 7.90 | 0.92 | 530 | 18 | 18 |
| Azulene | 7.08 | 0.49 | 7.02 | 0.29 | 408 | 18 | 18 |
| Benzoquinone | 9.59 | 1.50 | 9.66 | 1.35 | 298 | 18 | 18 |
| Naphthalenedione | 9.42 | 1.37 | 9.51 | 1.22 | 444 | 18 | 18 |
| Dichlone | 9.35 | 1.77 | 9.39 | 1.63 | 496 | 19 | 19 |
| tetrafluorobenzoquinone | 10.60 | 2.21 | 10.66 | 2.08 | 369 | 18 | 18 |
| tetrachlorobenzoquinone | 9.68 | 2.30 | 9.73 | 2.16 | 401 | 19 | 19 |
| Nitrobenzene | 9.76 | 0.44 | 9.77 | 0.27 | 341 | 17 | 17 |
| tetrafluorobenzenedicarbonitrile | 10.20 | 1.63 | 10.26 | 1.46 | 429 | 18 | 18 |
| Dinitrobenzonitrile | 10.70 | 1.63 | 10.73 | 1.47 | 468 | 18 | 18 |
| Nitrobenzonitrile | 10.17 | 1.23 | 10.18 | 1.07 | 389 | 17 | 17 |
| Benzonitrile | 9.48 | −0.23 | 9.45 | −0.43 | 310 | 17 | 17 |
| Fumaronitrile | 10.90 | 0.95 | 10.88 | 0.79 | 211 | 17 | 17 |
| mDCNB | 9.96 | 0.61 | 9.95 | 0.43 | 358 | 17 | 17 |
| TCNE | 11.34 | 3.04 | 11.37 | 2.91 | 309 | 18 | 18 |
| TCNQ | 8.98 | 3.39 | 8.95 | 3.26 | 543 | 18 | 18 |
| Maleicanhydride | 10.94 | 0.94 | 11.06 | 0.78 | 241 | 17 | 17 |
| Phthalimide | 9.86 | 0.56 | 9.98 | 0.39 | 401 | 17 | 17 |
| phthalicanhydride | 10.07 | 0.82 | 10.10 | 0.64 | 388 | 18 | 18 |
| tetrachloro-isobenzofuranedione | 9.59 | 1.53 | 9.63 | 1.36 | 491 | 19 | 19 |
| NDCA | 8.65 | 1.24 | 8.62 | 1.07 | 534 | 18 | 18 |
| bodipy | 7.73 | 1.56 | 7.66 | 1.39 | 516 | 16 | 16 |

TABLE VIII. Ionization potentials and electron affinities at the PBE0(+$G3W2$)/TZ3P level of theory (in eV) as well as total number of molecular orbitals and size of imaginary time and imaginary frequency grids for the acc24 test set.

### 8. $G_0W_0$(+$G3W2$)@PBE0/QZ6P

| | $GW$ | | $GW+G3W2$ | | | | |
|---|---|---|---|---|---|---|---|
| molecule | IP | EA | IP | EA | $N_{bas}$ | $N_{freq}$ | $N_{time}$ |
| Anthracene | 7.21 | 0.58 | 7.06 | 0.30 | 965 | 19 | 19 |
| Acridine | 7.73 | 0.90 | 7.60 | 0.63 | 946 | 19 | 19 |
| phenazine | 8.11 | 1.30 | 8.00 | 1.04 | 929 | 20 | 20 |
| Azulene | 7.25 | 0.69 | 7.13 | 0.41 | 713 | 19 | 19 |
| Benzoquinone | 9.85 | 1.67 | 9.88 | 1.45 | 515 | 20 | 20 |
| Naphthalenedione | 9.47 | 1.55 | 9.53 | 1.32 | 768 | 20 | 20 |
| Dichlone | 9.54 | 1.96 | 9.51 | 1.74 | 866 | 24 | 24 |
| tetrafluorobenzoquinone | 10.76 | 2.38 | 10.76 | 2.17 | 644 | 21 | 21 |
| tetrachlorobenzoquinone | 9.84 | 2.48 | 9.82 | 2.27 | 715 | 24 | 24 |
| Nitrobenzene | 10.08 | 0.64 | 10.02 | 0.39 | 595 | 20 | 20 |
| tetrafluorobenzenedicarbonitrile | 10.34 | 1.84 | 10.33 | 1.59 | 757 | 20 | 20 |
| Dinitrobenzonitrile | 10.84 | 1.81 | 10.82 | 1.57 | 813 | 20 | 20 |
| Nitrobenzonitrile | 10.27 | 1.42 | 10.22 | 1.18 | 678 | 20 | 20 |
| Benzonitrile | 9.64 | −0.02 | 9.55 | −0.29 | 542 | 19 | 19 |
| Fumaronitrile | 11.02 | 1.13 | 10.96 | 0.90 | 400 | 19 | 19 |
| mDCNB | 10.14 | 0.82 | 10.07 | 0.56 | 627 | 18 | 18 |
| TCNE | 11.49 | 3.22 | 11.48 | 3.01 | 539 | 18 | 18 |
| TCNQ | 9.15 | 3.56 | 9.06 | 3.35 | 940 | 19 | 19 |
| Maleicanhydride | 10.92 | 1.10 | 11.02 | 0.87 | 415 | 19 | 19 |
| Phthalimide | 9.79 | 0.76 | 9.88 | 0.51 | 695 | 20 | 20 |
| phthalicanhydride | 10.20 | 1.01 | 10.17 | 0.75 | 666 | 20 | 20 |
| tetrachloro-isobenzofuranedione | 9.68 | 1.74 | 9.65 | 1.49 | 862 | 24 | 24 |
| NDCA | 8.84 | 1.43 | 8.74 | 1.17 | 916 | 20 | 20 |
| bodipy | 7.92 | 1.73 | 7.76 | 1.46 | 913 | 21 | 21 |

TABLE IX. Ionization potentials and electron affinities at the PBE0(+$G3W2$)/QZ6P level of theory (in eV) as well as total number of molecular orbitals and size of imaginary time and imaginary frequency grids for the acc24 test set.

### 9. $G_0W_0$(+$G3W2$)@PBE/TZ3P

| molecule | $GW$ IP | $GW$ EA | $GW+G3W2$ IP | $GW+G3W2$ EA | $N_{bas}$ | $N_{freq}$ | $N_{time}$ |
|---|---|---|---|---|---|---|---|
| Anthracene | 6.75 | 0.48 | 6.68 | 0.27 | 555 | 18 | 18 |
| Acridine | 7.28 | 0.79 | 7.23 | 0.59 | 543 | 18 | 18 |
| phenazine | 8.08 | 1.16 | 8.10 | 0.98 | 530 | 18 | 18 |
| Azulene | 6.94 | 0.58 | 6.87 | 0.38 | 408 | 18 | 18 |
| Benzoquinone | 9.06 | 1.55 | 9.11 | 1.38 | 298 | 20 | 20 |
| Naphthalenedione | 8.45 | 1.45 | 8.50 | 1.27 | 444 | 20 | 20 |
| Dichlone | 8.70 | 1.81 | 8.80 | 1.64 | 496 | 21 | 21 |
| tetrafluorobenzoquinone | 10.09 | 2.17 | 10.15 | 2.01 | 369 | 19 | 19 |
| tetrachlorobenzoquinone | 9.26 | 2.28 | 9.30 | 2.13 | 401 | 21 | 21 |
| Nitrobenzene | 9.35 | 0.43 | 9.48 | 0.23 | 341 | 18 | 18 |
| tetrafluorobenzenedicarbonitrile | 9.71 | 1.60 | 9.76 | 1.42 | 429 | 18 | 18 |
| Dinitrobenzonitrile | 10.34 | 1.56 | 10.52 | 1.38 | 468 | 19 | 19 |
| Nitrobenzonitrile | 9.38 | 1.21 | 9.53 | 1.02 | 389 | 18 | 18 |
| Benzonitrile | 9.16 | −0.12 | 9.12 | −0.32 | 310 | 18 | 18 |
| Fumaronitrile | 10.51 | 1.04 | 10.51 | 0.86 | 211 | 16 | 16 |
| mDCNB | 9.59 | 0.68 | 9.57 | 0.49 | 358 | 18 | 18 |
| TCNE | 10.85 | 3.03 | 10.88 | 2.86 | 309 | 17 | 17 |
| TCNQ | 8.56 | 3.40 | 8.55 | 3.24 | 543 | 19 | 19 |
| Maleicanhydride | 10.12 | 1.00 | 10.20 | 0.82 | 241 | 19 | 19 |
| Phthalimide | 8.89 | 0.65 | 8.97 | 0.46 | 401 | 18 | 18 |
| phthalicanhydride | 9.51 | 0.88 | 9.61 | 0.69 | 388 | 18 | 18 |
| tetrachloro-isobenzofuranedione | 9.08 | 1.51 | 9.11 | 1.33 | 491 | 20 | 20 |
| NDCA | 8.33 | 1.28 | 8.30 | 1.10 | 534 | 19 | 19 |
| bodipy | 7.51 | 1.61 | 7.42 | 1.42 | 516 | 18 | 18 |

TABLE X. Ionization potentials and electron affinities at the PBE(+$G3W2$)/TZ3P level of theory (in eV) as well as total number of molecular orbitals and size of imaginary time and imaginary frequency grids for the acc24 test set.

### *10.* $G_0W_0(+G3W2)$*@PBE/QZ6P*

| | $GW$ | | $GW+G3W2$ | | | | |
|---|---|---|---|---|---|---|---|
| molecule | IP | EA | IP | EA | $N_{bas}$ | $N_{freq}$ | $N_{time}$ |
| Anthracene | 6.98 | 0.69 | 6.83 | 0.39 | 965 | 20 | 20 |
| Acridine | 7.40 | 0.99 | 7.27 | 0.70 | 946 | 21 | 21 |
| phenazine | 8.16 | 1.37 | 8.14 | 1.09 | 929 | 21 | 21 |
| Azulene | 7.02 | 0.78 | 6.88 | 0.49 | 713 | 21 | 21 |
| Benzoquinone | 8.91 | 1.73 | 8.91 | 1.48 | 515 | 22 | 22 |
| Naphthalenedione | 8.66 | 1.63 | 8.68 | 1.37 | 768 | 21 | 21 |
| Dichlone | 8.96 | 2.01 | 9.04 | 1.76 | 866 | 24 | 24 |
| tetrafluorobenzoquinone | 10.25 | 2.36 | 10.24 | 2.11 | 644 | 22 | 22 |
| tetrachlorobenzoquinone | 9.37 | 2.49 | 9.34 | 2.25 | 715 | 24 | 24 |
| Nitrobenzene | 9.70 | 0.64 | 9.81 | 0.35 | 595 | 21 | 21 |
| tetrafluorobenzenedicarbonitrile | 9.89 | 1.81 | 9.87 | 1.55 | 757 | 21 | 21 |
| Dinitrobenzonitrile | 10.65 | 1.75 | 10.83 | 1.49 | 813 | 21 | 21 |
| Nitrobenzonitrile | 10.28 | 1.41 | 10.43 | 1.14 | 678 | 21 | 21 |
| Benzonitrile | 9.28 | 0.10 | 9.18 | −0.19 | 542 | 19 | 19 |
| Fumaronitrile | 10.66 | 1.23 | 10.61 | 0.97 | 400 | 20 | 20 |
| mDCNB | 9.69 | 0.88 | 9.60 | 0.61 | 627 | 20 | 20 |
| TCNE | 10.97 | 3.20 | 10.96 | 2.96 | 539 | 19 | 19 |
| TCNQ | 8.76 | 3.57 | 8.67 | 3.32 | 940 | 22 | 22 |
| Maleicanhydride | 10.29 | 1.18 | 10.35 | 0.92 | 415 | 21 | 21 |
| Phthalimide | 9.32 | 0.85 | 9.38 | 0.58 | 695 | 21 | 21 |
| phthalicanhydride | 9.78 | 1.07 | 9.86 | 0.80 | 666 | 21 | 21 |
| tetrachloro-isobenzofuranedione | 9.26 | 1.73 | 9.22 | 1.46 | 862 | 24 | 24 |
| NDCA | 8.48 | 1.47 | 8.37 | 1.20 | 916 | 21 | 21 |
| bodipy | 7.63 | 1.79 | 7.47 | 1.50 | 913 | 23 | 23 |

TABLE XI. Ionization potentials and electron affinities at the PBE($+G3W2$)/QZ6P level of theory (in eV) as well as total number of molecular orbitals and size of imaginary time and imaginary frequency grids for the acc24 test set.

### B. Basis set limit extrapolated QP energies and comparison to CCSD(T) reference values

#### 1. *qsGW - ionization potentials*

| molecule | exp. | CC | $GW$ | $GW+G3W2$ | $GW$ - CC | $GW+G3W2$ - CC |
|---|---|---|---|---|---|---|
| Anthracene | 7.44 | 7.52 | 7.56 | 7.39 | 0.04 | −0.13 |
| Acridine | 7.80 | 8.04 | 8.02 | 7.87 | −0.02 | −0.17 |
| phenazine | 8.44 | 8.47 | 8.54 | 8.42 | 0.07 | −0.05 |
| Azulene | 7.42 | 7.55 | 7.65 | 7.52 | 0.10 | −0.03 |
| Benzoquinone | 10.00 | 10.27 | 10.70 | 10.73 | 0.43 | 0.46 |
| Naphthalenedione | 9.50 | 9.88 | 9.95 | 9.94 | 0.07 | 0.06 |
| Dichlone | 9.50 | 9.99 | 9.95 | 9.87 | −0.04 | −0.12 |
| tetrafluorobenzoquinone | 10.70 | 11.14 | 11.14 | 11.08 | 0.00 | −0.06 |
| tetrachlorobenzoquinone | 9.74 | 10.25 | 10.29 | 10.21 | 0.04 | −0.04 |
| Nitrobenzene | 9.94 | 10.19 | 10.22 | 10.16 | 0.03 | −0.03 |
| tetrafluorobenzenedicarbonitrile | 10.65 | 10.76 | 10.90 | 10.88 | 0.14 | 0.12 |
| Dinitrobenzonitrile | nan | 10.93 | 11.14 | 11.10 | 0.21 | 0.17 |
| Nitrobenzonitrile | 10.59 | 10.62 | 10.71 | 10.65 | 0.09 | 0.03 |
| Benzonitrile | 9.73 | 9.93 | 9.90 | 9.80 | −0.03 | −0.13 |
| Fumaronitrile | 11.30 | 11.48 | 11.43 | 11.33 | −0.05 | −0.15 |
| mDCNB | 10.20 | 10.45 | 10.43 | 10.34 | −0.02 | −0.11 |
| TCNE | 11.79 | 11.99 | 12.19 | 12.12 | 0.20 | 0.13 |
| TCNQ | nan | 9.57 | 9.60 | 9.44 | 0.03 | −0.13 |
| Maleicanhydride | 11.07 | 11.33 | 11.71 | 11.78 | 0.38 | 0.45 |
| Phthalimide | 9.90 | 10.08 | 10.15 | 10.10 | 0.07 | 0.02 |
| phthalicanhydride | 10.10 | 10.54 | 10.56 | 10.52 | 0.02 | −0.02 |
| tetrachloro-isobenzofuranedione | 10.80 | 10.05 | 10.00 | 9.94 | −0.05 | −0.11 |
| NDCA | 8.92 | 9.14 | 9.13 | 9.02 | −0.01 | −0.12 |
| bodipy | nan | 8.07 | 8.20 | 8.06 | 0.13 | −0.01 |
| MADs = | | | | | 0.09 | 0.12 |
| MDs = | | | | | 0.08 | 0.00 |
| MAXs = | | | | | 0.43 | 0.46 |
| r2 = | | | | | 0.99 | 0.99 |

TABLE XII. Ionization potentials for acc24: Experimental and CCSD(T) reference values and basis set limit extrapolated results for $GW$ and $GW+G3W2$ based on the qsGW starting point. The last three columns show deviations to the CCSD(T) reference values. Last for rows: Mean absolute deviations (MAD), mean signed deviations (MD), maximum errors (MAX), and Pearson correlation coefficients ($R^2$) All values are in eV.

*2. LRC-ωPBEh - ionization potentials*

| molecule | exp. | CC | $GW$ | $GW+G3W2$ | $GW$ - CC | $GW+G3W2$ - CC |
|---|---|---|---|---|---|---|
| Anthracene | 7.44 | 7.52 | 7.63 | 7.37 | 0.11 | −0.15 |
| Acridine | 7.80 | 8.04 | 8.10 | 7.88 | 0.06 | −0.16 |
| phenazine | 8.44 | 8.47 | 8.55 | 8.35 | 0.08 | −0.12 |
| Azulene | 7.42 | 7.55 | 7.66 | 7.45 | 0.11 | −0.10 |
| Benzoquinone | 10.00 | 10.27 | 10.56 | 10.60 | 0.29 | 0.33 |
| Naphthalenedione | 9.50 | 9.88 | 10.21 | 10.29 | 0.33 | 0.41 |
| Dichlone | 9.50 | 9.99 | 10.09 | 9.98 | 0.10 | −0.01 |
| tetrafluorobenzoquinone | 10.70 | 11.14 | 11.24 | 11.15 | 0.10 | 0.01 |
| tetrachlorobenzoquinone | 9.74 | 10.25 | 10.36 | 10.27 | 0.11 | 0.02 |
| Nitrobenzene | 9.94 | 10.19 | 10.27 | 10.15 | 0.08 | −0.04 |
| tetrafluorobenzenedicarbonitrile | 10.65 | 10.76 | 10.83 | 10.77 | 0.07 | 0.01 |
| Dinitrobenzonitrile | nan | 10.93 | 11.31 | 11.24 | 0.38 | 0.31 |
| Nitrobenzonitrile | 10.59 | 10.62 | 10.83 | 10.72 | 0.21 | 0.10 |
| Benzonitrile | 9.73 | 9.93 | 10.06 | 9.87 | 0.13 | −0.06 |
| Fumaronitrile | 11.30 | 11.48 | 11.52 | 11.39 | 0.04 | −0.09 |
| mDCNB | 10.20 | 10.45 | 10.65 | 10.50 | 0.20 | 0.05 |
| TCNE | 11.79 | 11.99 | 12.02 | 11.93 | 0.03 | −0.06 |
| TCNQ | nan | 9.57 | 9.69 | 9.47 | 0.12 | −0.10 |
| Maleicanhydride | 11.07 | 11.33 | 11.54 | 11.67 | 0.21 | 0.34 |
| Phthalimide | 9.90 | 10.08 | 10.49 | 10.62 | 0.41 | 0.54 |
| phthalicanhydride | 10.10 | 10.54 | 10.65 | 10.55 | 0.11 | 0.01 |
| tetrachloro-isobenzofuranedione | 10.80 | 10.05 | 10.19 | 10.10 | 0.14 | 0.05 |
| NDCA | 8.92 | 9.14 | 9.27 | 9.08 | 0.13 | −0.06 |
| bodipy | nan | 8.07 | 8.29 | 8.08 | 0.22 | 0.01 |
| MADs = | | | | | 0.16 | 0.13 |
| MDs = | | | | | 0.16 | 0.05 |
| MAXs = | | | | | 0.41 | 0.54 |
| r2 = | | | | | 0.99 | 0.98 |

TABLE XIII. Ionization potentials for acc24: Experimental and CCSD(T) reference values and basis set limit extrapolated results for $GW$ and $GW+G3W2$ based on the LRC-ωPBEh starting point. The last three columns show deviations to the CCSD(T) reference values. Last for rows: Mean absolute deviations (MAD), mean signed deviations (MD), maximum errors (MAX), and Pearson correlation coefficients ($R^2$) All values are in eV.

*3. ωB97-X - ionization potentials*

| molecule | exp. | CC | $GW$ | $GW + G3W2$ | $GW$ - CC | $GW + G3W2$ - CC |
|---|---|---|---|---|---|---|
| Anthracene | 7.44 | 7.52 | 7.68 | 7.43 | 0.16 | −0.09 |
| Acridine | 7.80 | 8.04 | 8.23 | 8.01 | 0.19 | −0.03 |
| phenazine | 8.44 | 8.47 | 8.65 | 8.47 | 0.18 | 0.00 |
| Azulene | 7.42 | 7.55 | 7.73 | 7.52 | 0.18 | −0.03 |
| Benzoquinone | 10.00 | 10.27 | 10.75 | 10.79 | 0.48 | 0.52 |
| Naphthalenedione | 9.50 | 9.88 | 10.14 | 10.07 | 0.26 | 0.19 |
| Dichlone | 9.50 | 9.99 | 10.22 | 10.12 | 0.23 | 0.13 |
| tetrafluorobenzoquinone | 10.70 | 11.14 | 11.40 | 11.32 | 0.26 | 0.18 |
| tetrachlorobenzoquinone | 9.74 | 10.25 | 10.50 | 10.42 | 0.25 | 0.17 |
| Nitrobenzene | 9.94 | 10.19 | 10.28 | 10.17 | 0.09 | −0.02 |
| tetrafluorobenzenedicarbonitrile | 10.65 | 10.76 | 10.97 | 10.91 | 0.21 | 0.15 |
| Dinitrobenzonitrile | nan | 10.93 | 11.47 | 11.40 | 0.54 | 0.47 |
| Nitrobenzonitrile | 10.59 | 10.62 | 10.86 | 10.75 | 0.24 | 0.13 |
| Benzonitrile | 9.73 | 9.93 | 10.29 | 10.13 | 0.36 | 0.20 |
| Fumaronitrile | 11.30 | 11.48 | 11.60 | 11.47 | 0.12 | −0.01 |
| mDCNB | 10.20 | 10.45 | 10.77 | 10.63 | 0.32 | 0.18 |
| TCNE | 11.79 | 11.99 | 12.18 | 12.08 | 0.19 | 0.09 |
| TCNQ | nan | 9.57 | 9.83 | 9.61 | 0.26 | 0.04 |
| Maleicanhydride | 11.07 | 11.33 | 11.76 | 11.90 | 0.43 | 0.57 |
| Phthalimide | 9.90 | 10.08 | 10.37 | 10.25 | 0.29 | 0.17 |
| phthalicanhydride | 10.10 | 10.54 | 10.74 | 10.65 | 0.20 | 0.11 |
| tetrachloro-isobenzofuranedione | 10.80 | 10.05 | 10.33 | 10.25 | 0.28 | 0.20 |
| NDCA | 8.92 | 9.14 | 9.38 | 9.20 | 0.24 | 0.06 |
| bodipy | nan | 8.07 | 8.40 | 8.17 | 0.33 | 0.10 |
| MADs = | | | | | 0.26 | 0.16 |
| MDs = | | | | | 0.26 | 0.14 |
| MAXs = | | | | | 0.54 | 0.57 |
| r2 = | | | | | 0.99 | 0.99 |

TABLE XIV. Ionization potentials for acc24: Experimental and CCSD(T) reference values and basis set limit extrapolated results for $GW$ and $GW + G3W2$ based on the $\omega$B97-X starting point. The last three columns show deviations to the CCSD(T) reference values. Last for rows: Mean absolute deviations (MAD), mean signed deviations (MD), maximum errors (MAX), and Pearson correlation coefficients ($R^2$) All values are in eV.

### 4. PBE0 - ionization potentials

| molecule | exp. | CC | $GW$ | $GW+G3W2$ | $GW$ - CC | $GW+G3W2$ - CC |
|---|---|---|---|---|---|---|
| Anthracene | 7.44 | 7.52 | 7.45 | 7.20 | −0.07 | −0.32 |
| Acridine | 7.80 | 8.04 | 8.01 | 7.79 | −0.03 | −0.25 |
| phenazine | 8.44 | 8.47 | 8.34 | 8.14 | −0.13 | −0.33 |
| Azulene | 7.42 | 7.55 | 7.49 | 7.27 | −0.06 | −0.28 |
| Benzoquinone | 10.00 | 10.27 | 10.19 | 10.19 | −0.08 | −0.08 |
| Naphthalenedione | 9.50 | 9.88 | 9.54 | 9.57 | −0.34 | −0.31 |
| Dichlone | 9.50 | 9.99 | 9.78 | 9.67 | −0.21 | −0.32 |
| tetrafluorobenzoquinone | 10.70 | 11.14 | 10.98 | 10.90 | −0.16 | −0.24 |
| tetrachlorobenzoquinone | 9.74 | 10.25 | 10.03 | 9.93 | −0.22 | −0.32 |
| Nitrobenzene | 9.94 | 10.19 | 10.51 | 10.36 | 0.32 | 0.17 |
| tetrafluorobenzenedicarbonitrile | 10.65 | 10.76 | 10.52 | 10.42 | −0.24 | −0.34 |
| Dinitrobenzonitrile | nan | 10.93 | 11.04 | 10.94 | 0.11 | 0.01 |
| Nitrobenzonitrile | 10.59 | 10.62 | 10.41 | 10.28 | −0.21 | −0.34 |
| Benzonitrile | 9.73 | 9.93 | 9.86 | 9.69 | −0.07 | −0.24 |
| Fumaronitrile | 11.30 | 11.48 | 11.16 | 11.05 | −0.32 | −0.43 |
| mDCNB | 10.20 | 10.45 | 10.37 | 10.22 | −0.08 | −0.23 |
| TCNE | 11.79 | 11.99 | 11.69 | 11.61 | −0.30 | −0.38 |
| TCNQ | nan | 9.57 | 9.38 | 9.21 | −0.19 | −0.36 |
| Maleicanhydride | 11.07 | 11.33 | 10.89 | 10.96 | −0.44 | −0.37 |
| Phthalimide | 9.90 | 10.08 | 9.68 | 9.73 | −0.40 | −0.35 |
| phthalicanhydride | 10.10 | 10.54 | 10.38 | 10.26 | −0.16 | −0.28 |
| tetrachloro-isobenzofuranedione | 10.80 | 10.05 | 9.79 | 9.68 | −0.26 | −0.37 |
| NDCA | 8.92 | 9.14 | 9.10 | 8.90 | −0.04 | −0.24 |
| bodipy | nan | 8.07 | 8.16 | 7.90 | 0.09 | −0.17 |
| MADs = | | | | | 0.19 | 0.28 |
| MDs = | | | | | −0.14 | −0.27 |
| MAXs = | | | | | 0.44 | 0.43 |
| r2 = | | | | | 0.98 | 0.99 |

TABLE XV. Ionization potentials for acc24: Experimental and CCSD(T) reference values and basis set limit extrapolated results for $GW$ and $GW+G3W2$ based on the PBE0 starting point. The last three columns show deviations to the CCSD(T) reference values. Last for rows: Mean absolute deviations (MAD), mean signed deviations (MD), maximum errors (MAX), and Pearson correlation coefficients ($R^2$) All values are in eV.

### 5. *PBE - ionization potentials*

| molecule | exp. | CC | $GW$ | $GW+G3W2$ | $GW$ - CC | $GW+G3W2$ - CC |
|---|---|---|---|---|---|---|
| Anthracene | 7.44 | 7.52 | 7.29 | 7.02 | −0.23 | −0.50 |
| Acridine | 7.80 | 8.04 | 7.56 | 7.33 | −0.48 | −0.71 |
| phenazine | 8.44 | 8.47 | 8.27 | 8.19 | −0.20 | −0.28 |
| Azulene | 7.42 | 7.55 | 7.13 | 6.90 | −0.42 | −0.65 |
| Benzoquinone | 10.00 | 10.27 | 8.69 | 8.62 | −1.58 | −1.65 |
| Naphthalenedione | 9.50 | 9.88 | 8.94 | 8.92 | −0.94 | −0.96 |
| Dichlone | 9.50 | 9.99 | 9.31 | 9.37 | −0.68 | −0.62 |
| tetrafluorobenzoquinone | 10.70 | 11.14 | 10.47 | 10.35 | −0.67 | −0.79 |
| tetrachlorobenzoquinone | 9.74 | 10.25 | 9.50 | 9.40 | −0.75 | −0.85 |
| Nitrobenzene | 9.94 | 10.19 | 10.17 | 10.24 | −0.02 | 0.05 |
| tetrafluorobenzenedicarbonitrile | 10.65 | 10.76 | 10.13 | 10.02 | −0.63 | −0.74 |
| Dinitrobenzonitrile | nan | 10.93 | 11.07 | 11.24 | 0.14 | 0.31 |
| Nitrobenzonitrile | 10.59 | 10.62 | 11.49 | 11.64 | 0.87 | 1.02 |
| Benzonitrile | 9.73 | 9.93 | 9.44 | 9.26 | −0.49 | −0.67 |
| Fumaronitrile | 11.30 | 11.48 | 10.83 | 10.73 | −0.65 | −0.75 |
| mDCNB | 10.20 | 10.45 | 9.83 | 9.65 | −0.62 | −0.80 |
| TCNE | 11.79 | 11.99 | 11.13 | 11.07 | −0.86 | −0.92 |
| TCNQ | nan | 9.57 | 9.01 | 8.84 | −0.56 | −0.73 |
| Maleicanhydride | 11.07 | 11.33 | 10.53 | 10.56 | −0.80 | −0.77 |
| Phthalimide | 9.90 | 10.08 | 9.91 | 9.95 | −0.17 | −0.13 |
| phthalicanhydride | 10.10 | 10.54 | 10.16 | 10.21 | −0.38 | −0.33 |
| tetrachloro-isobenzofuranedione | 10.80 | 10.05 | 9.49 | 9.37 | −0.56 | −0.68 |
| NDCA | 8.92 | 9.14 | 8.69 | 8.47 | −0.45 | −0.67 |
| bodipy | nan | 8.07 | 7.79 | 7.53 | −0.28 | −0.54 |
| MADs = | | | | | 0.56 | 0.67 |
| MDs = | | | | | −0.47 | −0.56 |
| MAXs = | | | | | 1.58 | 1.65 |
| r2 = | | | | | 0.87 | 0.86 |

TABLE XVI. Ionization potentials for acc24: Experimental and CCSD(T) reference values and basis set limit extrapolated results for $GW$ and $GW+G3W2$ based on the PBE starting point. The last three columns show deviations to the CCSD(T) reference values. Last for rows: Mean absolute deviations (MAD), mean signed deviations (MD), maximum errors (MAX), and Pearson correlation coefficients ($R^2$) All values are in eV.

### 6. qs$GW$ - electron affinities

| molecule | exp. | CC | $GW$ | $GW+G3W2$ | $GW$ - CC | $GW+G3W2$ - CC |
|---|---|---|---|---|---|---|
| Anthracene | 0.53 | 0.33 | 0.58 | 0.31 | 0.25 | −0.02 |
| Acridine | 0.90 | 0.69 | 0.89 | 0.64 | 0.20 | −0.05 |
| phenazine | 1.31 | 1.11 | 1.31 | 1.07 | 0.20 | −0.04 |
| Azulene | 0.80 | 0.54 | 0.72 | 0.44 | 0.18 | −0.10 |
| Benzoquinone | 1.85 | 1.55 | 1.63 | 1.44 | 0.08 | −0.11 |
| Naphthalenedione | 1.81 | 1.47 | 1.60 | 1.39 | 0.13 | −0.08 |
| Dichlone | 2.21 | 1.92 | 1.95 | 1.75 | 0.03 | −0.17 |
| tetrafluorobenzoquinone | 2.70 | 2.29 | 2.42 | 2.24 | 0.13 | −0.05 |
| tetrachlorobenzoquinone | 2.78 | 2.48 | 2.45 | 2.26 | −0.03 | −0.22 |
| Nitrobenzene | 1.00 | 0.54 | 0.73 | 0.51 | 0.19 | −0.03 |
| tetrafluorobenzenedicarbonitrile | 1.89 | 1.62 | 1.86 | 1.62 | 0.24 | 0.00 |
| Dinitrobenzonitrile | 2.16 | 1.76 | 1.94 | 1.72 | 0.18 | −0.04 |
| Nitrobenzonitrile | 1.69 | 1.30 | 1.48 | 1.26 | 0.18 | −0.04 |
| Benzonitrile | 0.26 | −0.21 | 0.00 | −0.26 | 0.21 | −0.05 |
| Fumaronitrile | 1.25 | 0.98 | 1.03 | 0.84 | 0.05 | −0.14 |
| mDCNB | 0.91 | 0.61 | 0.81 | 0.56 | 0.20 | −0.05 |
| TCNE | 3.16 | 3.05 | 3.27 | 3.09 | 0.22 | 0.04 |
| TCNQ | 2.80 | 3.33 | 3.50 | 3.33 | 0.17 | 0.00 |
| Maleicanhydride | 1.44 | 1.01 | 1.07 | 0.86 | 0.06 | −0.15 |
| Phthalimide | 1.02 | 0.63 | 0.76 | 0.51 | 0.13 | −0.12 |
| phthalicanhydride | 1.25 | 0.87 | 0.99 | 0.74 | 0.12 | −0.13 |
| tetrachloro-isobenzofuranedione | 1.96 | 1.68 | 1.71 | 1.46 | 0.03 | −0.22 |
| NDCA | nan | 1.26 | 1.40 | 1.16 | 0.14 | −0.10 |
| bodipy | nan | 1.67 | 1.72 | 1.50 | 0.05 | −0.17 |
| MADs = | | | | | 0.14 | 0.09 |
| MDs = | | | | | 0.14 | −0.09 |
| MAXs = | | | | | 0.25 | 0.23 |
| r2 = | | | | | 0.99 | 0.99 |

TABLE XVII. Electron Affinities for acc24: Experimental and CCSD(T) reference values and basis set limit extrapolated results for $GW$ and $GW+G3W2$ based on the qsGW starting point. The last three columns show deviations to the CCSD(T) reference values. Last for rows: Mean absolute deviations (MAD), mean signed deviations (MD), maximum errors (MAX), and Pearson correlation coefficients ($R^2$) All values are in eV.

### 7. LRC-ωPBEh - electron affinities

| molecule | exp. | CC | $GW$ | $GW+G3W2$ | $GW$ - CC | $GW+G3W2$ - CC |
|---|---|---|---|---|---|---|
| Anthracene | 0.53 | 0.33 | 0.68 | 0.29 | 0.35 | −0.04 |
| Acridine | 0.90 | 0.69 | 1.01 | 0.64 | 0.32 | −0.05 |
| phenazine | 1.31 | 1.11 | 1.42 | 1.06 | 0.31 | −0.05 |
| Azulene | 0.80 | 0.54 | 0.83 | 0.44 | 0.29 | −0.10 |
| Benzoquinone | 1.85 | 1.55 | 1.74 | 1.45 | 0.19 | −0.10 |
| Naphthalenedione | 1.81 | 1.47 | 1.70 | 1.39 | 0.23 | −0.08 |
| Dichlone | 2.21 | 1.92 | 2.14 | 1.83 | 0.22 | −0.09 |
| tetrafluorobenzoquinone | 2.70 | 2.29 | 2.54 | 2.26 | 0.25 | −0.03 |
| tetrachlorobenzoquinone | 2.78 | 2.48 | 2.65 | 2.36 | 0.17 | −0.12 |
| Nitrobenzene | 1.00 | 0.54 | 0.83 | 0.49 | 0.29 | −0.05 |
| tetrafluorobenzenedicarbonitrile | 1.89 | 1.62 | 1.97 | 1.64 | 0.35 | 0.02 |
| Dinitrobenzonitrile | 2.16 | 1.76 | 2.03 | 1.70 | 0.27 | −0.06 |
| Nitrobenzonitrile | 1.69 | 1.30 | 1.63 | 1.31 | 0.33 | 0.01 |
| Benzonitrile | 0.26 | −0.21 | 0.11 | −0.26 | 0.32 | −0.05 |
| Fumaronitrile | 1.25 | 0.98 | 1.20 | 0.92 | 0.22 | −0.06 |
| mDCNB | 0.91 | 0.61 | 0.95 | 0.59 | 0.34 | −0.02 |
| TCNE | 3.16 | 3.05 | 3.36 | 3.09 | 0.31 | 0.04 |
| TCNQ | 2.80 | 3.33 | 3.69 | 3.41 | 0.36 | 0.08 |
| Maleicanhydride | 1.44 | 1.01 | 1.22 | 0.91 | 0.21 | −0.10 |
| Phthalimide | 1.02 | 0.63 | 0.90 | 0.55 | 0.27 | −0.08 |
| phthalicanhydride | 1.25 | 0.87 | 1.14 | 0.79 | 0.27 | −0.08 |
| tetrachloro-isobenzofuranedione | 1.96 | 1.68 | 1.90 | 1.55 | 0.22 | −0.13 |
| NDCA | nan | 1.26 | 1.56 | 1.19 | 0.30 | −0.07 |
| bodipy | nan | 1.67 | 1.83 | 1.47 | 0.16 | −0.20 |
| MADs = | | | | | 0.27 | 0.07 |
| MDs = | | | | | 0.27 | −0.06 |
| MAXs = | | | | | 0.36 | 0.20 |
| r2 = | | | | | 1.00 | 1.00 |

TABLE XVIII. Electron Affinities for acc24: Experimental and CCSD(T) reference values and basis set limit extrapolated results for $GW$ and $GW+G3W2$ based on the LRC-ωPBEh starting point. The last three columns show deviations to the CCSD(T) reference values. Last for rows: Mean absolute deviations (MAD), mean signed deviations (MD), maximum errors (MAX), and Pearson correlation coefficients ($R^2$) All values are in eV.

### *8. ωB97-X - electron affinities*

| molecule | exp. | CC | $GW$ | $GW + G3W2$ | $GW$ - CC | $GW + G3W2$ - CC |
|---|---|---|---|---|---|---|
| Anthracene | 0.53 | 0.33 | 0.71 | 0.33 | 0.38 | 0.00 |
| Acridine | 0.90 | 0.69 | 1.04 | 0.67 | 0.35 | −0.02 |
| phenazine | 1.31 | 1.11 | 1.44 | 1.10 | 0.33 | −0.01 |
| Azulene | 0.80 | 0.54 | 0.88 | 0.50 | 0.34 | −0.04 |
| Benzoquinone | 1.85 | 1.55 | 1.78 | 1.50 | 0.23 | −0.05 |
| Naphthalenedione | 1.81 | 1.47 | 1.72 | 1.41 | 0.25 | −0.06 |
| Dichlone | 2.21 | 1.92 | 2.15 | 1.85 | 0.23 | −0.07 |
| tetrafluorobenzoquinone | 2.70 | 2.29 | 2.55 | 2.28 | 0.26 | −0.01 |
| tetrachlorobenzoquinone | 2.78 | 2.48 | 2.66 | 2.39 | 0.18 | −0.09 |
| Nitrobenzene | 1.00 | 0.54 | 0.86 | 0.53 | 0.32 | −0.01 |
| tetrafluorobenzenedicarbonitrile | 1.89 | 1.62 | 1.98 | 1.65 | 0.36 | 0.03 |
| Dinitrobenzonitrile | 2.16 | 1.76 | 2.08 | 1.77 | 0.32 | 0.01 |
| Nitrobenzonitrile | 1.69 | 1.30 | 1.64 | 1.33 | 0.34 | 0.03 |
| Benzonitrile | 0.26 | −0.21 | 0.13 | −0.23 | 0.34 | −0.02 |
| Fumaronitrile | 1.25 | 0.98 | 1.20 | 0.92 | 0.22 | −0.06 |
| mDCNB | 0.91 | 0.61 | 0.96 | 0.61 | 0.35 | 0.00 |
| TCNE | 3.16 | 3.05 | 3.36 | 3.09 | 0.31 | 0.04 |
| TCNQ | 2.80 | 3.33 | 3.70 | 3.43 | 0.37 | 0.10 |
| Maleicanhydride | 1.44 | 1.01 | 1.22 | 0.92 | 0.21 | −0.09 |
| Phthalimide | 1.02 | 0.63 | 0.92 | 0.57 | 0.29 | −0.06 |
| phthalicanhydride | 1.25 | 0.87 | 1.17 | 0.82 | 0.30 | −0.05 |
| tetrachloro-isobenzofuranedione | 1.96 | 1.68 | 1.94 | 1.60 | 0.26 | −0.08 |
| NDCA | nan | 1.26 | 1.57 | 1.22 | 0.31 | −0.04 |
| bodipy | nan | 1.67 | 1.87 | 1.52 | 0.20 | −0.15 |
| MADs = | | | | | 0.29 | 0.05 |
| MDs = | | | | | 0.29 | −0.03 |
| MAXs = | | | | | 0.38 | 0.15 |
| r2 = | | | | | 1.00 | 1.00 |

TABLE XIX. Electron Affinities for acc24: Experimental and CCSD(T) reference values and basis set limit extrapolated results for $GW$ and $GW+G3W2$ based on the ωB97-X starting point. The last three columns show deviations to the CCSD(T) reference values. Last for rows: Mean absolute deviations (MAD), mean signed deviations (MD), maximum errors (MAX), and Pearson correlation coefficients ($R^2$) All values are in eV.

*9. PBE0 - electron affinities*

| molecule | exp. | CC | $GW$ | $GW + G3W2$ | $GW$ - CC | $GW + G3W2$ - CC |
|---|---|---|---|---|---|---|
| Anthracene | 0.53 | 0.33 | 0.87 | 0.47 | 0.54 | 0.14 |
| Acridine | 0.90 | 0.69 | 1.18 | 0.79 | 0.49 | 0.10 |
| phenazine | 1.31 | 1.11 | 1.57 | 1.19 | 0.46 | 0.08 |
| Azulene | 0.80 | 0.54 | 0.95 | 0.56 | 0.41 | 0.02 |
| Benzoquinone | 1.85 | 1.55 | 1.90 | 1.57 | 0.35 | 0.02 |
| Naphthalenedione | 1.81 | 1.47 | 1.80 | 1.45 | 0.33 | −0.02 |
| Dichlone | 2.21 | 1.92 | 2.22 | 1.88 | 0.30 | −0.04 |
| tetrafluorobenzoquinone | 2.70 | 2.29 | 2.62 | 2.30 | 0.33 | 0.01 |
| tetrachlorobenzoquinone | 2.78 | 2.48 | 2.72 | 2.40 | 0.24 | −0.08 |
| Nitrobenzene | 1.00 | 0.54 | 0.91 | 0.55 | 0.37 | 0.01 |
| tetrafluorobenzenedicarbonitrile | 1.89 | 1.62 | 2.11 | 1.76 | 0.49 | 0.14 |
| Dinitrobenzonitrile | 2.16 | 1.76 | 2.06 | 1.71 | 0.30 | −0.05 |
| Nitrobenzonitrile | 1.69 | 1.30 | 1.68 | 1.32 | 0.38 | 0.02 |
| Benzonitrile | 0.26 | −0.21 | 0.26 | −0.11 | 0.47 | 0.10 |
| Fumaronitrile | 1.25 | 0.98 | 1.34 | 1.03 | 0.36 | 0.05 |
| mDCNB | 0.91 | 0.61 | 1.11 | 0.73 | 0.50 | 0.12 |
| TCNE | 3.16 | 3.05 | 3.46 | 3.14 | 0.41 | 0.09 |
| TCNQ | 2.80 | 3.33 | 3.78 | 3.46 | 0.45 | 0.13 |
| Maleicanhydride | 1.44 | 1.01 | 1.34 | 1.00 | 0.33 | −0.01 |
| Phthalimide | 1.02 | 0.63 | 1.04 | 0.66 | 0.41 | 0.03 |
| phthalicanhydride | 1.25 | 0.87 | 1.27 | 0.91 | 0.40 | 0.04 |
| tetrachloro-isobenzofuranedione | 1.96 | 1.68 | 2.01 | 1.65 | 0.33 | −0.03 |
| NDCA | nan | 1.26 | 1.69 | 1.31 | 0.43 | 0.05 |
| bodipy | nan | 1.67 | 1.95 | 1.56 | 0.28 | −0.11 |
| MADs = | | | | | 0.39 | 0.06 |
| MDs = | | | | | 0.39 | 0.03 |
| MAXs = | | | | | 0.54 | 0.14 |
| r2 = | | | | | 0.99 | 0.99 |

TABLE XX. Electron Affinities for acc24: Experimental and CCSD(T) reference values and basis set limit extrapolated results for $GW$ and $GW + G3W2$ based on the PBE0 starting point. The last three columns show deviations to the CCSD(T) reference values. Last for rows: Mean absolute deviations (MAD), mean signed deviations (MD), maximum errors (MAX), and Pearson correlation coefficients ($R^2$) All values are in eV.

### *10. PBE - electron affinities*

| molecule | exp. | CC | $GW$ | $GW+G3W2$ | $GW$ - CC | $GW+G3W2$ - CC |
|---|---|---|---|---|---|---|
| Anthracene | 0.53 | 0.33 | 0.97 | 0.55 | 0.64 | 0.22 |
| Acridine | 0.90 | 0.69 | 1.27 | 0.86 | 0.58 | 0.17 |
| phenazine | 1.31 | 1.11 | 1.64 | 1.24 | 0.53 | 0.13 |
| Azulene | 0.80 | 0.54 | 1.04 | 0.65 | 0.50 | 0.11 |
| Benzoquinone | 1.85 | 1.55 | 1.98 | 1.61 | 0.43 | 0.06 |
| Naphthalenedione | 1.81 | 1.47 | 1.89 | 1.51 | 0.42 | 0.04 |
| Dichlone | 2.21 | 1.92 | 2.28 | 1.92 | 0.36 | 0.00 |
| tetrafluorobenzoquinone | 2.70 | 2.29 | 2.61 | 2.26 | 0.32 | −0.03 |
| tetrachlorobenzoquinone | 2.78 | 2.48 | 2.76 | 2.41 | 0.28 | −0.07 |
| Nitrobenzene | 1.00 | 0.54 | 0.92 | 0.51 | 0.38 | −0.03 |
| tetrafluorobenzenedicarbonitrile | 1.89 | 1.62 | 2.08 | 1.71 | 0.46 | 0.09 |
| Dinitrobenzonitrile | 2.16 | 1.76 | 2.02 | 1.63 | 0.26 | −0.13 |
| Nitrobenzonitrile | 1.69 | 1.30 | 1.67 | 1.30 | 0.37 | 0.00 |
| Benzonitrile | 0.26 | −0.21 | 0.38 | −0.02 | 0.59 | 0.19 |
| Fumaronitrile | 1.25 | 0.98 | 1.43 | 1.09 | 0.45 | 0.11 |
| mDCNB | 0.91 | 0.61 | 1.16 | 0.77 | 0.55 | 0.16 |
| TCNE | 3.16 | 3.05 | 3.44 | 3.09 | 0.39 | 0.04 |
| TCNQ | 2.80 | 3.33 | 3.79 | 3.43 | 0.46 | 0.10 |
| Maleicanhydride | 1.44 | 1.01 | 1.43 | 1.06 | 0.42 | 0.05 |
| Phthalimide | 1.02 | 0.63 | 1.13 | 0.75 | 0.50 | 0.12 |
| phthalicanhydride | 1.25 | 0.87 | 1.34 | 0.95 | 0.47 | 0.08 |
| tetrachloro-isobenzofuranedione | 1.96 | 1.68 | 2.02 | 1.64 | 0.34 | −0.04 |
| NDCA | nan | 1.26 | 1.74 | 1.34 | 0.48 | 0.08 |
| bodipy | nan | 1.67 | 2.02 | 1.61 | 0.35 | −0.06 |
| MADs = | | | | | 0.44 | 0.09 |
| MDs = | | | | | 0.44 | 0.06 |
| MAXs = | | | | | 0.64 | 0.22 |
| r2 = | | | | | 0.99 | 0.99 |

TABLE XXI. Electron Affinities for acc24: Experimental and CCSD(T) reference values and basis set limit extrapolated results for $GW$ and $GW+G3W2$ based on the PBE starting point. The last three columns show deviations to the CCSD(T) reference values. Last for rows: Mean absolute deviations (MAD), mean signed deviations (MD), maximum errors (MAX), and Pearson correlation coefficients ($R^2$) All values are in eV.

### *11. qsGW - fundamental gaps*

| molecule | exp. | CC | $GW$ | $GW+G3W2$ | $GW$ - CC | $GW+G3W2$ - CC |
|---|---|---|---|---|---|---|
| Anthracene | 6.91 | 7.19 | 6.98 | 7.08 | −0.21 | −0.11 |
| Acridine | 6.90 | 7.35 | 7.12 | 7.24 | −0.23 | −0.11 |
| phenazine | 7.13 | 7.36 | 7.23 | 7.35 | −0.13 | −0.01 |
| Azulene | 6.62 | 7.01 | 6.93 | 7.08 | −0.08 | 0.07 |
| Benzoquinone | 8.15 | 8.72 | 9.07 | 9.29 | 0.35 | 0.57 |
| Naphthalenedione | 7.69 | 8.41 | 8.35 | 8.54 | −0.06 | 0.13 |
| Dichlone | 7.29 | 8.07 | 7.99 | 8.13 | −0.08 | 0.06 |
| tetrafluorobenzoquinone | 8.00 | 8.85 | 8.72 | 8.84 | −0.13 | −0.01 |
| tetrachlorobenzoquinone | 6.96 | 7.77 | 7.84 | 7.96 | 0.07 | 0.19 |
| Nitrobenzene | 8.94 | 9.65 | 9.48 | 9.66 | −0.17 | 0.01 |
| tetrafluorobenzenedicarbonitrile | 8.76 | 9.14 | 9.04 | 9.26 | −0.10 | 0.12 |
| Dinitrobenzonitrile | nan | 9.17 | 9.20 | 9.38 | 0.03 | 0.21 |
| Nitrobenzonitrile | 8.90 | 9.32 | 9.23 | 9.39 | −0.09 | 0.07 |
| Benzonitrile | 9.47 | 10.14 | 9.91 | 10.07 | −0.23 | −0.07 |
| Fumaronitrile | 10.05 | 10.50 | 10.40 | 10.48 | −0.10 | −0.02 |
| mDCNB | 9.29 | 9.84 | 9.62 | 9.79 | −0.22 | −0.05 |
| TCNE | 8.63 | 8.94 | 8.93 | 9.03 | −0.01 | 0.09 |
| TCNQ | nan | 6.24 | 6.11 | 6.11 | −0.13 | −0.13 |
| Maleicanhydride | 9.63 | 10.32 | 10.64 | 10.92 | 0.32 | 0.60 |
| Phthalimide | 8.88 | 9.45 | 9.39 | 9.58 | −0.06 | 0.13 |
| phthalicanhydride | 8.85 | 9.67 | 9.57 | 9.78 | −0.10 | 0.11 |
| tetrachloro-isobenzofuranedione | 8.84 | 8.37 | 8.29 | 8.48 | −0.08 | 0.11 |
| NDCA | nan | 7.88 | 7.73 | 7.86 | −0.15 | −0.02 |
| bodipy | nan | 6.40 | 6.48 | 6.56 | 0.08 | 0.16 |
| MADs = | | | | | 0.13 | 0.13 |
| MDs = | | | | | −0.06 | 0.09 |
| MAXs = | | | | | 0.35 | 0.60 |
| r2 = | | | | | 0.99 | 0.98 |

TABLE XXII. Fundamental Gaps for acc24: Experimental and CCSD(T) reference values and basis set limit extrapolated results for $GW$ and $GW+G3W2$ based on the qsGW starting point. The last three columns show deviations to the CCSD(T) reference values. Last for rows: Mean absolute deviations (MAD), mean signed deviations (MD), maximum errors (MAX), and Pearson correlation coefficients ($R^2$) All values are in eV.

### 12. LRC-$\omega$PBEh - fundamental gaps

| molecule | exp. | CC | $GW$ | $GW+G3W2$ | $GW$ - CC | $GW+G3W2$ - CC |
|---|---|---|---|---|---|---|
| Anthracene | 6.91 | 7.19 | 6.94 | 7.08 | −0.25 | −0.11 |
| Acridine | 6.90 | 7.35 | 7.09 | 7.24 | −0.26 | −0.11 |
| phenazine | 7.13 | 7.36 | 7.13 | 7.29 | −0.23 | −0.07 |
| Azulene | 6.62 | 7.01 | 6.83 | 7.01 | −0.18 | 0.00 |
| Benzoquinone | 8.15 | 8.72 | 8.82 | 9.15 | 0.10 | 0.43 |
| Naphthalenedione | 7.69 | 8.41 | 8.50 | 8.90 | 0.09 | 0.49 |
| Dichlone | 7.29 | 8.07 | 7.95 | 8.15 | −0.12 | 0.08 |
| tetrafluorobenzoquinone | 8.00 | 8.85 | 8.70 | 8.89 | −0.15 | 0.04 |
| tetrachlorobenzoquinone | 6.96 | 7.77 | 7.71 | 7.90 | −0.06 | 0.13 |
| Nitrobenzene | 8.94 | 9.65 | 9.44 | 9.66 | −0.21 | 0.01 |
| tetrafluorobenzenedicarbonitrile | 8.76 | 9.14 | 8.87 | 9.13 | −0.27 | −0.01 |
| Dinitrobenzonitrile | nan | 9.17 | 9.29 | 9.54 | 0.12 | 0.37 |
| Nitrobenzonitrile | 8.90 | 9.32 | 9.19 | 9.41 | −0.13 | 0.09 |
| Benzonitrile | 9.47 | 10.14 | 9.95 | 10.13 | −0.19 | −0.01 |
| Fumaronitrile | 10.05 | 10.50 | 10.32 | 10.47 | −0.18 | −0.03 |
| mDCNB | 9.29 | 9.84 | 9.70 | 9.92 | −0.14 | 0.08 |
| TCNE | 8.63 | 8.94 | 8.66 | 8.85 | −0.28 | −0.09 |
| TCNQ | nan | 6.24 | 6.00 | 6.06 | −0.24 | −0.18 |
| Maleicanhydride | 9.63 | 10.32 | 10.32 | 10.76 | 0.00 | 0.44 |
| Phthalimide | 8.88 | 9.45 | 9.60 | 10.07 | 0.15 | 0.62 |
| phthalicanhydride | 8.85 | 9.67 | 9.51 | 9.76 | −0.16 | 0.09 |
| tetrachloro-isobenzofuranedione | 8.84 | 8.37 | 8.29 | 8.55 | −0.08 | 0.18 |
| NDCA | nan | 7.88 | 7.71 | 7.89 | −0.17 | 0.01 |
| bodipy | nan | 6.40 | 6.46 | 6.61 | 0.06 | 0.21 |
| MADs = | | | | | 0.16 | 0.16 |
| MDs = | | | | | −0.12 | 0.11 |
| MAXs = | | | | | 0.28 | 0.62 |
| r2 = | | | | | 0.99 | 0.98 |

TABLE XXIII. Fundamental Gaps for acc24: Experimental and CCSD(T) reference values and basis set limit extrapolated results for $GW$ and $GW+G3W2$ based on the LRC-$\omega$PBEh starting point. The last three columns show deviations to the CCSD(T) reference values. Last for rows: Mean absolute deviations (MAD), mean signed deviations (MD), maximum errors (MAX), and Pearson correlation coefficients ($R^2$) All values are in eV.

### *13. ωB97-X - fundamental gaps*

| molecule | exp. | CC | $GW$ | $GW+G3W2$ | $GW$ - CC | $GW+G3W2$ - CC |
|---|---|---|---|---|---|---|
| Anthracene | 6.91 | 7.19 | 6.98 | 7.11 | −0.21 | −0.08 |
| Acridine | 6.90 | 7.35 | 7.18 | 7.33 | −0.17 | −0.02 |
| phenazine | 7.13 | 7.36 | 7.21 | 7.37 | −0.15 | 0.01 |
| Azulene | 6.62 | 7.01 | 6.85 | 7.02 | −0.16 | 0.01 |
| Benzoquinone | 8.15 | 8.72 | 8.97 | 9.29 | 0.25 | 0.57 |
| Naphthalenedione | 7.69 | 8.41 | 8.43 | 8.66 | 0.02 | 0.25 |
| Dichlone | 7.29 | 8.07 | 8.07 | 8.27 | 0.00 | 0.20 |
| tetrafluorobenzoquinone | 8.00 | 8.85 | 8.85 | 9.05 | 0.00 | 0.20 |
| tetrachlorobenzoquinone | 6.96 | 7.77 | 7.84 | 8.03 | 0.07 | 0.26 |
| Nitrobenzene | 8.94 | 9.65 | 9.42 | 9.63 | −0.23 | −0.02 |
| tetrafluorobenzenedicarbonitrile | 8.76 | 9.14 | 8.99 | 9.26 | −0.15 | 0.12 |
| Dinitrobenzonitrile | nan | 9.17 | 9.39 | 9.62 | 0.22 | 0.45 |
| Nitrobenzonitrile | 8.90 | 9.32 | 9.21 | 9.42 | −0.11 | 0.10 |
| Benzonitrile | 9.47 | 10.14 | 10.15 | 10.36 | 0.01 | 0.22 |
| Fumaronitrile | 10.05 | 10.50 | 10.40 | 10.54 | −0.10 | 0.04 |
| mDCNB | 9.29 | 9.84 | 9.81 | 10.02 | −0.03 | 0.18 |
| TCNE | 8.63 | 8.94 | 8.82 | 8.99 | −0.12 | 0.05 |
| TCNQ | nan | 6.24 | 6.14 | 6.18 | −0.10 | −0.06 |
| Maleicanhydride | 9.63 | 10.32 | 10.54 | 10.98 | 0.22 | 0.66 |
| Phthalimide | 8.88 | 9.45 | 9.45 | 9.68 | 0.00 | 0.23 |
| phthalicanhydride | 8.85 | 9.67 | 9.57 | 9.83 | −0.10 | 0.16 |
| tetrachloro-isobenzofuranedione | 8.84 | 8.37 | 8.39 | 8.64 | 0.02 | 0.27 |
| NDCA | nan | 7.88 | 7.81 | 7.98 | −0.07 | 0.10 |
| bodipy | nan | 6.40 | 6.53 | 6.65 | 0.13 | 0.25 |
| MADs = | | | | | 0.11 | 0.19 |
| MDs = | | | | | −0.03 | 0.17 |
| MAXs = | | | | | 0.25 | 0.66 |
| r2 = | | | | | 0.99 | 0.98 |

TABLE XXIV. Fundamental Gaps for acc24: Experimental and CCSD(T) reference values and basis set limit extrapolated results for $GW$ and $GW+G3W2$ based on the ωB97-X starting point. The last three columns show deviations to the CCSD(T) reference values. Last for rows: Mean absolute deviations (MAD), mean signed deviations (MD), maximum errors (MAX), and Pearson correlation coefficients ($R^2$) All values are in eV.

### *14. PBE0 - fundamental gaps*

| molecule | exp. | CC | $GW$ | $GW+G3W2$ | $GW$ - CC | $GW+G3W2$ - CC |
|---|---|---|---|---|---|---|
| Anthracene | 6.91 | 7.19 | 6.58 | 6.73 | −0.61 | −0.46 |
| Acridine | 6.90 | 7.35 | 6.82 | 7.00 | −0.53 | −0.35 |
| phenazine | 7.13 | 7.36 | 6.78 | 6.95 | −0.58 | −0.41 |
| Azulene | 6.62 | 7.01 | 6.54 | 6.71 | −0.47 | −0.30 |
| Benzoquinone | 8.15 | 8.72 | 8.29 | 8.61 | −0.43 | −0.11 |
| Naphthalenedione | 7.69 | 8.41 | 7.75 | 8.11 | −0.66 | −0.30 |
| Dichlone | 7.29 | 8.07 | 7.57 | 7.79 | −0.50 | −0.28 |
| tetrafluorobenzoquinone | 8.00 | 8.85 | 8.36 | 8.60 | −0.49 | −0.25 |
| tetrachlorobenzoquinone | 6.96 | 7.77 | 7.32 | 7.54 | −0.45 | −0.23 |
| Nitrobenzene | 8.94 | 9.65 | 9.60 | 9.81 | −0.05 | 0.16 |
| tetrafluorobenzenedicarbonitrile | 8.76 | 9.14 | 8.40 | 8.66 | −0.74 | −0.48 |
| Dinitrobenzonitrile | nan | 9.17 | 8.97 | 9.22 | −0.20 | 0.05 |
| Nitrobenzonitrile | 8.90 | 9.32 | 8.73 | 8.96 | −0.59 | −0.36 |
| Benzonitrile | 9.47 | 10.14 | 9.60 | 9.80 | −0.54 | −0.34 |
| Fumaronitrile | 10.05 | 10.50 | 9.82 | 10.02 | −0.68 | −0.48 |
| mDCNB | 9.29 | 9.84 | 9.27 | 9.49 | −0.57 | −0.35 |
| TCNE | 8.63 | 8.94 | 8.23 | 8.47 | −0.71 | −0.47 |
| TCNQ | nan | 6.24 | 5.60 | 5.75 | −0.64 | −0.49 |
| Maleicanhydride | 9.63 | 10.32 | 9.55 | 9.96 | −0.77 | −0.36 |
| Phthalimide | 8.88 | 9.45 | 8.64 | 9.07 | −0.81 | −0.38 |
| phthalicanhydride | 8.85 | 9.67 | 9.11 | 9.36 | −0.56 | −0.31 |
| tetrachloro-isobenzofuranedione | 8.84 | 8.37 | 7.78 | 8.03 | −0.59 | −0.34 |
| NDCA | nan | 7.88 | 7.41 | 7.59 | −0.47 | −0.29 |
| bodipy | nan | 6.40 | 6.21 | 6.34 | −0.19 | −0.06 |
| MADs = | | | | | 0.54 | 0.32 |
| MDs = | | | | | −0.54 | −0.30 |
| MAXs = | | | | | 0.81 | 0.49 |
| r2 = | | | | | 0.98 | 0.98 |

TABLE XXV. Fundamental Gaps for acc24: Experimental and CCSD(T) reference values and basis set limit extrapolated results for $GW$ and $GW+G3W2$ based on the PBE0 starting point. The last three columns show deviations to the CCSD(T) reference values. Last for rows: Mean absolute deviations (MAD), mean signed deviations (MD), maximum errors (MAX), and Pearson correlation coefficients ($R^2$) All values are in eV.

*15. PBE - fundamental gaps*

| molecule | exp. | CC | $GW$ | $GW+G3W2$ | $GW$ - CC | $GW+G3W2$ - CC |
|---|---|---|---|---|---|---|
| Anthracene | 6.91 | 7.19 | 6.32 | 6.47 | −0.87 | −0.72 |
| Acridine | 6.90 | 7.35 | 6.29 | 6.47 | −1.06 | −0.88 |
| phenazine | 7.13 | 7.36 | 6.63 | 6.95 | −0.73 | −0.41 |
| Azulene | 6.62 | 7.01 | 6.09 | 6.25 | −0.92 | −0.76 |
| Benzoquinone | 8.15 | 8.72 | 6.71 | 7.01 | −2.01 | −1.71 |
| Naphthalenedione | 7.69 | 8.41 | 7.06 | 7.41 | −1.35 | −1.00 |
| Dichlone | 7.29 | 8.07 | 7.02 | 7.44 | −1.05 | −0.63 |
| tetrafluorobenzoquinone | 8.00 | 8.85 | 7.86 | 8.09 | −0.99 | −0.76 |
| tetrachlorobenzoquinone | 6.96 | 7.77 | 6.74 | 6.99 | −1.03 | −0.78 |
| Nitrobenzene | 8.94 | 9.65 | 9.26 | 9.73 | −0.39 | 0.08 |
| tetrafluorobenzenedicarbonitrile | 8.76 | 9.14 | 8.05 | 8.31 | −1.09 | −0.83 |
| Dinitrobenzonitrile | nan | 9.17 | 9.05 | 9.61 | −0.12 | 0.44 |
| Nitrobenzonitrile | 8.90 | 9.32 | 9.82 | 10.34 | 0.50 | 1.02 |
| Benzonitrile | 9.47 | 10.14 | 9.06 | 9.28 | −1.08 | −0.86 |
| Fumaronitrile | 10.05 | 10.50 | 9.40 | 9.64 | −1.10 | −0.86 |
| mDCNB | 9.29 | 9.84 | 8.67 | 8.88 | −1.17 | −0.96 |
| TCNE | 8.63 | 8.94 | 7.69 | 7.98 | −1.25 | −0.96 |
| TCNQ | nan | 6.24 | 5.22 | 5.41 | −1.02 | −0.83 |
| Maleicanhydride | 9.63 | 10.32 | 9.10 | 9.50 | −1.22 | −0.82 |
| Phthalimide | 8.88 | 9.45 | 8.78 | 9.20 | −0.67 | −0.25 |
| phthalicanhydride | 8.85 | 9.67 | 8.82 | 9.26 | −0.85 | −0.41 |
| tetrachloro-isobenzofuranedione | 8.84 | 8.37 | 7.47 | 7.73 | −0.90 | −0.64 |
| NDCA | nan | 7.88 | 6.95 | 7.13 | −0.93 | −0.75 |
| bodipy | nan | 6.40 | 5.77 | 5.92 | −0.63 | −0.48 |
| MADs = | | | | | 0.95 | 0.74 |
| MDs = | | | | | −0.91 | −0.61 |
| MAXs = | | | | | 2.01 | 1.71 |
| r2 = | | | | | 0.88 | 0.86 |

TABLE XXVI. Fundamental Gaps for acc24: Experimental and CCSD(T) reference values and basis set limit extrapolated results for $GW$ and $GW+G3W2$ based on the PBE starting point. The last three columns show deviations to the CCSD(T) reference values. Last for rows: Mean absolute deviations (MAD), mean signed deviations (MD), maximum errors (MAX), and Pearson correlation coefficients ($R^2$) All values are in eV.

# III. IONIZATION POTENTIALS FOR 40 SMALL MOLECULES (GW40)

## A. Individual QP energies and technical parameters

### 1. qsGW(+G3W2)/TZ3P

| | $GW$ | | $GW+G3W2$ | | | | |
|---|---|---|---|---|---|---|---|
| molecule | IP | EA | IP | EA | $N_{bas}$ | $N_{freq}$ | $N_{time}$ |
| C2F4 | 10.73 | −1.95 | 10.66 | −1.96 | 186 | 18 | 14 |
| CF4 | 16.73 | −2.27 | 17.08 | −2.28 | 155 | 16 | 13 |
| SiF4 | 16.79 | −1.31 | 17.15 | −1.31 | 163 | 21 | 16 |
| HCN | 13.56 | −2.24 | 13.60 | −2.27 | 76 | 17 | 14 |
| C2H2 | 11.25 | −2.54 | 11.23 | −2.57 | 90 | 18 | 13 |
| HCCF | 11.33 | −1.98 | 11.30 | −2.00 | 107 | 18 | 14 |
| HCCCN | 11.52 | −1.11 | 11.49 | −1.24 | 138 | 18 | 15 |
| NNO | 12.89 | −2.89 | 12.96 | −3.07 | 93 | 17 | 15 |
| C2N2 | 13.45 | −0.41 | 13.48 | −0.52 | 124 | 16 | 14 |
| CO | 14.25 | −2.60 | 14.35 | −2.68 | 62 | 18 | 15 |
| CO2 | 13.99 | −4.14 | 14.11 | −4.30 | 93 | 17 | 14 |
| C3O2 | 10.77 | −0.71 | 10.76 | −0.87 | 155 | 17 | 15 |
| OCS | 11.12 | −1.92 | 11.16 | −2.07 | 101 | 23 | 17 |
| FCN | 13.53 | −1.35 | 13.56 | −1.37 | 93 | 17 | 14 |
| N2 | 15.73 | −3.21 | 15.89 | −3.33 | 62 | 16 | 13 |
| HC4H | 10.12 | −1.73 | 10.05 | −1.86 | 152 | 17 | 14 |
| HCl | 12.58 | −1.65 | 12.72 | −1.67 | 53 | 23 | 17 |
| HF | 16.36 | −1.63 | 16.72 | −1.64 | 45 | 17 | 13 |
| F2 | 16.20 | 0.09 | 16.55 | 0.05 | 62 | 16 | 13 |
| SiO | 11.55 | −0.39 | 11.62 | −0.45 | 70 | 22 | 15 |
| CS | 11.40 | −0.70 | 11.50 | −0.81 | 70 | 22 | 16 |
| P2 | 10.23 | 0.16 | 10.25 | 0.07 | 78 | 22 | 17 |
| H2CO | 11.18 | −1.66 | 11.25 | −1.77 | 90 | 17 | 15 |
| H2O | 12.89 | −1.63 | 13.11 | −1.65 | 59 | 17 | 16 |
| C2H4 | 10.51 | −2.43 | 10.46 | −2.47 | 118 | 17 | 14 |
| H2CS | 9.30 | −0.12 | 9.35 | −0.23 | 98 | 22 | 17 |
| HCONH2 | 10.75 | −1.73 | 10.89 | −1.77 | 135 | 17 | 15 |
| HCOOH | 11.84 | −1.97 | 11.98 | −2.00 | 121 | 17 | 16 |
| NSF | 11.80 | 0.54 | 11.91 | 0.43 | 101 | 23 | 16 |
| O3 | 13.13 | 1.87 | 13.40 | 1.85 | 93 | 17 | 15 |
| C2H2F2 | 10.68 | −2.13 | 10.63 | −2.15 | 152 | 17 | 13 |
| cisC2H2F2 | 10.56 | −2.04 | 10.52 | −2.07 | 152 | 18 | 14 |
| CH4 | 14.57 | −2.31 | 14.60 | −2.33 | 87 | 15 | 13 |
| CH3CCH | 10.43 | −2.06 | 10.38 | −2.09 | 149 | 17 | 13 |
| CH3CN | 12.48 | −1.63 | 12.49 | −1.66 | 135 | 16 | 14 |
| CH3NC | 11.67 | −1.82 | 11.81 | −1.85 | 135 | 16 | 14 |
| CH3F | 13.70 | −2.27 | 13.79 | −2.29 | 104 | 17 | 13 |
| CH2F2 | 13.88 | −2.28 | 13.93 | −2.31 | 121 | 17 | 13 |
| CHF3 | 15.38 | −2.27 | 15.48 | −2.30 | 138 | 17 | 13 |
| C2H6 | 12.97 | −2.29 | 12.91 | −2.32 | 146 | 15 | 13 |

TABLE XXVII. Ionization potentials and electron affinities at the qsGW(+$G3W2$)/TZ3P level of theory (in eV) as well as total number of molecular orbitals and size of imaginary time and imaginary frequency grids for the gw40 test set.

### 2. qsGW(+G3W2)/QZ6P

| | $GW$ | | $GW+G3W2$ | | | | |
|---|---|---|---|---|---|---|---|
| molecule | IP | EA | IP | EA | $N_{bas}$ | $N_{freq}$ | $N_{time}$ |
| C2F4 | 10.79 | −2.59 | 10.66 | −2.64 | 354 | 18 | 14 |
| CF4 | 16.78 | −2.94 | 17.05 | −2.97 | 299 | 16 | 13 |
| SiF4 | 16.85 | −1.90 | 17.15 | −1.91 | 316 | 21 | 16 |
| HCN | 13.66 | −1.52 | 13.68 | −1.55 | 145 | 17 | 14 |
| C2H2 | 11.38 | −1.94 | 11.34 | −1.96 | 168 | 18 | 13 |
| HCCF | 11.42 | −1.77 | 11.36 | −1.79 | 200 | 18 | 14 |
| HCCCN | 11.75 | −0.89 | 11.69 | −1.05 | 255 | 18 | 15 |
| NNO | 12.88 | −1.61 | 12.94 | −1.64 | 178 | 17 | 15 |
| C2N2 | 13.52 | −0.19 | 13.52 | −0.34 | 232 | 16 | 14 |
| CO | 14.28 | −2.29 | 14.40 | −2.41 | 111 | 18 | 15 |
| CO2 | 14.04 | −1.44 | 14.15 | −1.47 | 167 | 17 | 14 |
| C3O2 | 10.95 | −0.55 | 10.90 | −0.74 | 277 | 17 | 15 |
| OCS | 11.28 | −1.09 | 11.29 | −1.11 | 184 | 23 | 17 |
| FCN | 13.67 | −1.27 | 13.66 | −1.32 | 177 | 17 | 14 |
| N2 | 15.88 | −2.26 | 16.05 | −2.28 | 122 | 16 | 13 |
| HC4H | 10.23 | −1.47 | 10.14 | −1.64 | 278 | 17 | 14 |
| HCl | 12.69 | −1.18 | 12.79 | −1.20 | 107 | 23 | 17 |
| HF | 16.48 | −1.36 | 16.79 | −1.37 | 90 | 17 | 13 |
| F2 | 16.38 | 0.07 | 16.67 | −0.03 | 122 | 16 | 13 |
| SiO | 11.61 | −0.12 | 11.67 | −0.19 | 128 | 22 | 15 |
| CS | 11.64 | −0.33 | 11.75 | −0.48 | 128 | 22 | 16 |
| P2 | 10.31 | 0.39 | 10.31 | 0.26 | 154 | 22 | 17 |
| H2CO | 11.23 | −1.46 | 11.28 | −1.59 | 169 | 17 | 15 |
| H2O | 12.87 | −1.28 | 13.10 | −1.30 | 114 | 17 | 16 |
| C2H4 | 10.60 | −1.68 | 10.53 | −1.71 | 226 | 17 | 14 |
| H2CS | 9.43 | 0.08 | 9.45 | −0.06 | 186 | 22 | 17 |
| HCONH2 | 10.79 | −1.17 | 10.92 | −1.20 | 259 | 17 | 15 |
| HCOOH | 11.83 | −1.54 | 11.95 | −1.57 | 225 | 17 | 16 |
| NSF | 11.99 | 0.80 | 12.08 | 0.66 | 195 | 23 | 16 |
| O3 | 13.24 | 1.98 | 13.49 | 1.91 | 168 | 17 | 15 |
| C2H2F2 | 10.76 | −1.60 | 10.68 | −1.63 | 290 | 17 | 13 |
| cisC2H2F2 | 10.64 | −1.48 | 10.56 | −1.50 | 290 | 18 | 14 |
| CH4 | 14.61 | −1.59 | 14.62 | −1.61 | 171 | 15 | 13 |
| CH3CCH | 10.54 | −1.47 | 10.47 | −1.49 | 281 | 17 | 13 |
| CH3CN | 12.57 | −1.19 | 12.55 | −1.21 | 258 | 16 | 14 |
| CH3NC | 11.79 | −1.23 | 11.93 | −1.26 | 258 | 16 | 14 |
| CH3F | 13.70 | −1.58 | 13.76 | −1.60 | 203 | 17 | 13 |
| CH2F2 | 13.90 | −1.60 | 13.91 | −1.62 | 235 | 17 | 13 |
| CHF3 | 15.39 | −1.71 | 15.45 | −1.73 | 267 | 17 | 13 |
| C2H6 | 13.01 | −1.57 | 12.94 | −1.60 | 284 | 15 | 13 |

TABLE XXVIII. Ionization potentials and electron affinities at the qsGW(+$G3W2$)/QZ6P level of theory (in eV) as well as total number of molecular orbitals and size of imaginary time and imaginary frequency grids for the gw40 test set.

### 3. $G_0W_0$(+$G3W2$)@LRC-$\omega$PBEh/TZ3P

| | $GW$ | | $GW+G3W2$ | | | | |
|---|---|---|---|---|---|---|---|
| molecule | IP | EA | IP | EA | $N_{bas}$ | $N_{freq}$ | $N_{time}$ |
| C2F4 | 10.35 | −1.95 | 10.30 | −1.97 | 186 | 18 | 14 |
| CF4 | 16.16 | −2.26 | 16.49 | −2.26 | 155 | 16 | 13 |
| SiF4 | 16.30 | −1.35 | 16.64 | −1.36 | 163 | 21 | 16 |
| HCN | 13.56 | −3.10 | 13.59 | −3.24 | 76 | 17 | 14 |
| C2H2 | 11.28 | −2.40 | 11.27 | −2.44 | 90 | 18 | 13 |
| HCCF | 11.23 | −1.92 | 11.21 | −1.94 | 107 | 18 | 14 |
| HCCCN | 11.60 | −0.94 | 11.58 | −1.09 | 138 | 18 | 15 |
| NNO | 12.75 | −2.83 | 12.82 | −3.05 | 93 | 17 | 15 |
| C2N2 | 13.32 | −0.26 | 13.35 | −0.40 | 124 | 16 | 14 |
| CO | 14.07 | −2.57 | 14.16 | −2.70 | 62 | 18 | 15 |
| CO2 | 13.74 | −4.17 | 13.84 | −4.38 | 93 | 17 | 14 |
| C3O2 | 10.72 | −0.70 | 10.71 | −0.88 | 155 | 17 | 15 |
| OCS | 11.05 | −1.84 | 11.09 | −2.01 | 101 | 23 | 17 |
| FCN | 13.41 | −1.38 | 13.44 | −1.41 | 93 | 17 | 14 |
| N2 | 15.59 | −3.06 | 15.71 | −3.22 | 62 | 16 | 13 |
| HC4H | 10.11 | −1.56 | 10.05 | −1.71 | 152 | 17 | 14 |
| HCl | 12.41 | −1.70 | 12.54 | −1.74 | 53 | 23 | 17 |
| HF | 15.93 | −1.68 | 16.25 | −1.69 | 45 | 17 | 13 |
| F2 | 15.68 | −0.14 | 15.99 | −0.24 | 62 | 16 | 13 |
| SiO | 11.45 | −0.45 | 11.52 | −0.52 | 70 | 22 | 15 |
| CS | 11.57 | −0.53 | 11.66 | −0.67 | 70 | 22 | 16 |
| P2 | 10.19 | 0.18 | 10.22 | 0.08 | 78 | 22 | 17 |
| H2CO | 10.98 | −1.61 | 11.05 | −1.76 | 90 | 17 | 15 |
| H2O | 12.61 | −1.64 | 12.80 | −1.66 | 59 | 17 | 16 |
| C2H4 | 10.48 | −2.62 | 10.44 | −2.77 | 118 | 17 | 14 |
| H2CS | 9.22 | −0.07 | 9.25 | −0.20 | 98 | 22 | 17 |
| HCONH2 | 10.45 | −1.66 | 10.58 | −1.70 | 135 | 17 | 15 |
| HCOOH | 11.54 | −2.59 | 11.67 | −2.78 | 121 | 17 | 16 |
| NSF | 11.70 | 0.54 | 11.80 | 0.41 | 101 | 23 | 16 |
| O3 | 12.81 | 1.69 | 13.03 | 1.60 | 93 | 17 | 15 |
| C2H2F2 | 10.47 | −2.10 | 10.43 | −2.13 | 152 | 17 | 13 |
| cisC2H2F2 | 10.33 | −2.08 | 10.30 | −2.12 | 152 | 18 | 14 |
| CH4 | 14.37 | −2.26 | 14.40 | −2.28 | 87 | 15 | 13 |
| CH3CCH | 10.39 | −1.93 | 10.34 | −1.97 | 149 | 17 | 13 |
| CH3CN | 12.39 | −1.58 | 12.40 | −1.62 | 135 | 16 | 14 |
| CH3NC | 11.49 | −1.71 | 11.63 | −1.74 | 135 | 16 | 14 |
| CH3F | 13.36 | −2.23 | 13.48 | −2.26 | 104 | 17 | 13 |
| CH2F2 | 13.50 | −2.23 | 13.57 | −2.27 | 121 | 17 | 13 |
| CHF3 | 14.93 | −2.24 | 15.04 | −2.27 | 138 | 17 | 13 |
| C2H6 | 12.82 | −2.23 | 12.77 | −2.27 | 146 | 15 | 13 |

TABLE XXIX. Ionization potentials and electron affinities at the LRC-$\omega$PBEh(+$G3W2$)/TZ3P level of theory (in eV) as well as total number of molecular orbitals and size of imaginary time and imaginary frequency grids for the gw40 test set.

### 4. $G_0W_0$(+$G3W2$)@LRC-$\omega$PBEh/QZ6P

| | *GW* | | *GW* + *G*3*W*2 | | | | |
|---|---|---|---|---|---|---|---|
| molecule | IP | EA | IP | EA | $N_{bas}$ | $N_{freq}$ | $N_{time}$ |
| C2F4 | 10.54 | 0.91 | 10.44 | 0.87 | 354 | 18 | 14 |
| CF4 | 16.35 | 0.81 | 16.70 | 0.74 | 299 | 16 | 13 |
| SiF4 | 16.46 | 0.07 | 16.96 | 0.06 | 316 | 21 | 16 |
| HCN | 13.67 | −1.45 | 13.68 | −1.47 | 145 | 17 | 14 |
| C2H2 | 11.38 | −1.75 | 11.33 | −1.78 | 168 | 18 | 13 |
| HCCF | 11.37 | −1.62 | 11.31 | −1.66 | 200 | 18 | 14 |
| HCCCN | 11.72 | −0.73 | 11.66 | −0.95 | 255 | 18 | 15 |
| NNO | 12.89 | −2.54 | 12.93 | −2.81 | 178 | 17 | 15 |
| C2N2 | 13.51 | −0.06 | 13.50 | −0.27 | 232 | 16 | 14 |
| CO | 14.14 | −2.19 | 14.24 | −2.36 | 111 | 18 | 15 |
| CO2 | 13.88 | −1.29 | 13.99 | −1.33 | 167 | 17 | 14 |
| C3O2 | 10.91 | −0.50 | 10.85 | −0.74 | 277 | 17 | 15 |
| OCS | 11.20 | −1.55 | 11.20 | −1.78 | 184 | 23 | 17 |
| FCN | 13.54 | −1.19 | 13.54 | −1.27 | 177 | 17 | 14 |
| N2 | 15.72 | −2.64 | 15.87 | −2.84 | 122 | 16 | 13 |
| HC4H | 10.23 | −1.31 | 10.12 | −1.53 | 278 | 17 | 14 |
| HCl | 12.58 | −0.84 | 12.68 | −0.87 | 107 | 23 | 17 |
| HF | 16.05 | −1.19 | 16.36 | −1.20 | 90 | 17 | 13 |
| F2 | 15.90 | 0.10 | 16.16 | −0.06 | 122 | 16 | 13 |
| SiO | 11.54 | −0.15 | 11.63 | −0.26 | 128 | 22 | 15 |
| CS | 11.63 | −0.23 | 11.74 | −0.42 | 128 | 22 | 16 |
| P2 | 10.29 | 0.39 | 10.29 | 0.23 | 154 | 22 | 17 |
| H2CO | 11.10 | −1.34 | 11.13 | −1.54 | 169 | 17 | 15 |
| H2O | 12.68 | −1.16 | 12.89 | −1.18 | 114 | 17 | 16 |
| C2H4 | 10.59 | −2.31 | 10.50 | −2.52 | 226 | 17 | 14 |
| H2CS | 9.37 | 0.12 | 9.36 | −0.07 | 186 | 22 | 17 |
| HCONH2 | 10.55 | −1.07 | 10.67 | −1.11 | 259 | 17 | 15 |
| HCOOH | 11.65 | −1.40 | 11.78 | −1.44 | 225 | 17 | 16 |
| NSF | 11.88 | 0.78 | 12.00 | 0.59 | 195 | 23 | 16 |
| O3 | 12.98 | 1.93 | 13.22 | 1.78 | 168 | 17 | 15 |
| C2H2F2 | 10.62 | −1.34 | 10.54 | −1.37 | 290 | 17 | 13 |
| cisC2H2F2 | 10.51 | −1.42 | 10.42 | −1.46 | 290 | 18 | 14 |
| CH4 | 14.48 | −1.55 | 14.49 | −1.58 | 171 | 15 | 13 |
| CH3CCH | 10.45 | −1.38 | 10.36 | −1.41 | 281 | 17 | 13 |
| CH3CN | 12.51 | −1.05 | 12.48 | −1.09 | 258 | 16 | 14 |
| CH3NC | 11.61 | −1.11 | 11.74 | −1.14 | 258 | 16 | 14 |
| CH3F | 13.49 | −1.51 | 13.57 | −1.54 | 203 | 17 | 13 |
| CH2F2 | 13.62 | −1.53 | 13.64 | −1.56 | 235 | 17 | 13 |
| CHF3 | 15.06 | −1.55 | 15.14 | −1.58 | 267 | 17 | 13 |
| C2H6 | 12.89 | −1.51 | 12.80 | −1.54 | 284 | 15 | 13 |

TABLE XXX. Ionization potentials and electron affinities at the LRC-$\omega$PBEh(+$G3W2$)/QZ6P level of theory (in eV) as well as total number of molecular orbitals and size of imaginary time and imaginary frequency grids for the gw40 test set.

### 5. $G_0W_0(+G3W2)$@$\omega$B97-X/TZ3P

| | $GW$ | | $GW+G3W2$ | | | | |
|---|---|---|---|---|---|---|---|
| molecule | IP | EA | IP | EA | $N_{bas}$ | $N_{freq}$ | $N_{time}$ |
| C2F4 | 10.46 | −1.96 | 10.40 | −1.98 | 186 | 18 | 14 |
| CF4 | 16.27 | −2.27 | 16.61 | −2.28 | 155 | 16 | 13 |
| SiF4 | 16.41 | −1.36 | 16.77 | −1.37 | 163 | 21 | 16 |
| HCN | 13.62 | −3.10 | 13.64 | −3.23 | 76 | 17 | 14 |
| C2H2 | 11.34 | −2.52 | 11.32 | −2.55 | 90 | 18 | 13 |
| HCCF | 11.29 | −1.93 | 11.28 | −1.96 | 107 | 18 | 14 |
| HCCCN | 11.67 | −0.98 | 11.65 | −1.12 | 138 | 18 | 15 |
| NNO | 12.78 | −2.86 | 12.85 | −3.07 | 93 | 17 | 15 |
| C2N2 | 13.41 | −0.28 | 13.45 | −0.41 | 124 | 16 | 14 |
| CO | 14.17 | −2.56 | 14.27 | −2.68 | 62 | 18 | 15 |
| CO2 | 13.83 | −4.19 | 13.94 | −4.39 | 93 | 17 | 14 |
| C3O2 | 10.76 | −0.71 | 10.75 | −0.88 | 155 | 17 | 15 |
| OCS | 11.09 | −1.84 | 11.13 | −2.02 | 101 | 23 | 17 |
| FCN | 13.45 | −1.39 | 13.49 | −1.42 | 93 | 17 | 14 |
| N2 | 15.67 | −3.10 | 15.80 | −3.25 | 62 | 16 | 13 |
| HC4H | 10.16 | −1.60 | 10.10 | −1.75 | 152 | 17 | 14 |
| HCl | 12.44 | −1.70 | 12.57 | −1.74 | 53 | 23 | 17 |
| HF | 16.02 | −1.68 | 16.36 | −1.69 | 45 | 17 | 13 |
| F2 | 15.77 | −0.17 | 16.10 | −0.25 | 62 | 16 | 13 |
| SiO | 11.50 | −0.41 | 11.57 | −0.48 | 70 | 22 | 15 |
| CS | 11.68 | −0.50 | 11.78 | −0.63 | 70 | 22 | 16 |
| P2 | 10.22 | 0.19 | 10.25 | 0.09 | 78 | 22 | 17 |
| H2CO | 11.06 | −1.64 | 11.13 | −1.78 | 90 | 17 | 15 |
| H2O | 12.69 | −1.65 | 12.90 | −1.67 | 59 | 17 | 16 |
| C2H4 | 10.53 | −2.63 | 10.49 | −2.77 | 118 | 17 | 14 |
| H2CS | 9.26 | −0.06 | 9.30 | −0.18 | 98 | 22 | 17 |
| HCONH2 | 10.57 | −1.68 | 10.71 | −1.72 | 135 | 17 | 15 |
| HCOOH | 11.64 | −2.61 | 11.78 | −2.79 | 121 | 17 | 16 |
| NSF | 11.82 | 0.55 | 11.93 | 0.42 | 101 | 23 | 16 |
| O3 | 12.89 | 1.70 | 13.13 | 1.63 | 93 | 17 | 15 |
| C2H2F2 | 10.55 | −2.12 | 10.51 | −2.15 | 152 | 17 | 13 |
| cisC2H2F2 | 10.42 | −2.08 | 10.39 | −2.11 | 152 | 18 | 14 |
| CH4 | 14.50 | −2.28 | 14.54 | −2.30 | 87 | 15 | 13 |
| CH3CCH | 10.46 | −1.96 | 10.41 | −2.00 | 149 | 17 | 13 |
| CH3CN | 12.47 | −1.60 | 12.48 | −1.63 | 135 | 16 | 14 |
| CH3NC | 11.65 | −1.74 | 11.80 | −1.77 | 135 | 16 | 14 |
| CH3F | 13.45 | −2.24 | 13.57 | −2.27 | 104 | 17 | 13 |
| CH2F2 | 13.60 | −2.24 | 13.67 | −2.28 | 121 | 17 | 13 |
| CHF3 | 15.03 | −2.25 | 15.15 | −2.28 | 138 | 17 | 13 |
| C2H6 | 12.91 | −2.26 | 12.86 | −2.29 | 146 | 15 | 13 |

TABLE XXXI. Ionization potentials and electron affinities at the $\omega$B97-X($+G3W2$)/TZ3P level of theory (in eV) as well as total number of molecular orbitals and size of imaginary time and imaginary frequency grids for the gw40 test set.

### 6. $G_0W_0(+G3W2)$@$\omega$B97-X/QZ6P

| | $GW$ | | $GW+G3W2$ | | | | |
|---|---|---|---|---|---|---|---|
| molecule | IP | EA | IP | EA | $N_{bas}$ | $N_{freq}$ | $N_{time}$ |
| C2F4 | 10.65 | 1.04 | 10.55 | 1.00 | 354 | 18 | 14 |
| CF4 | 16.46 | 1.11 | 16.83 | 1.03 | 299 | 16 | 13 |
| SiF4 | 16.59 | 0.14 | 17.11 | 0.14 | 316 | 21 | 16 |
| HCN | 13.73 | −1.45 | 13.75 | −1.47 | 145 | 17 | 14 |
| C2H2 | 11.45 | −1.77 | 11.40 | −1.79 | 168 | 18 | 13 |
| HCCF | 11.43 | −1.62 | 11.37 | −1.66 | 200 | 18 | 14 |
| HCCCN | 11.80 | −0.76 | 11.74 | −0.97 | 255 | 18 | 15 |
| NNO | 12.94 | −2.56 | 12.99 | −2.83 | 178 | 17 | 15 |
| C2N2 | 13.57 | −0.07 | 13.56 | −0.27 | 232 | 16 | 14 |
| CO | 14.26 | −2.17 | 14.37 | −2.33 | 111 | 18 | 15 |
| CO2 | 13.95 | −1.30 | 14.08 | −1.34 | 167 | 17 | 14 |
| C3O2 | 10.95 | −0.49 | 10.90 | −0.73 | 277 | 17 | 15 |
| OCS | 11.25 | −1.55 | 11.25 | −1.77 | 184 | 23 | 17 |
| FCN | 13.61 | −1.20 | 13.61 | −1.27 | 177 | 17 | 14 |
| N2 | 15.86 | −2.67 | 16.02 | −2.87 | 122 | 16 | 13 |
| HC4H | 10.30 | −1.34 | 10.19 | −1.55 | 278 | 17 | 14 |
| HCl | 12.63 | −0.83 | 12.75 | −0.85 | 107 | 23 | 17 |
| HF | 16.15 | −1.18 | 16.48 | −1.20 | 90 | 17 | 13 |
| F2 | 16.00 | 0.07 | 16.28 | −0.08 | 122 | 16 | 13 |
| SiO | 11.61 | −0.11 | 11.70 | −0.21 | 128 | 22 | 15 |
| CS | 11.81 | −0.20 | 11.93 | −0.38 | 128 | 22 | 16 |
| P2 | 10.33 | 0.40 | 10.33 | 0.25 | 154 | 22 | 17 |
| H2CO | 11.18 | −1.35 | 11.22 | −1.53 | 169 | 17 | 15 |
| H2O | 12.74 | −1.16 | 12.96 | −1.18 | 114 | 17 | 16 |
| C2H4 | 10.65 | −1.64 | 10.57 | −1.68 | 226 | 17 | 14 |
| H2CS | 9.42 | 0.14 | 9.43 | −0.04 | 186 | 22 | 17 |
| HCONH2 | 10.68 | −1.09 | 10.80 | −1.13 | 259 | 17 | 15 |
| HCOOH | 11.76 | −1.42 | 11.91 | −1.45 | 225 | 17 | 16 |
| NSF | 11.99 | 0.79 | 12.11 | 0.61 | 195 | 23 | 16 |
| O3 | 13.21 | 1.95 | 13.46 | 1.82 | 168 | 17 | 15 |
| C2H2F2 | 10.79 | −1.36 | 10.71 | −1.40 | 290 | 17 | 13 |
| cisC2H2F2 | 10.60 | −1.42 | 10.52 | −1.46 | 290 | 18 | 14 |
| CH4 | 14.58 | −1.57 | 14.59 | −1.59 | 171 | 15 | 13 |
| CH3CCH | 10.61 | −1.40 | 10.51 | −1.44 | 281 | 17 | 13 |
| CH3CN | 12.59 | −1.07 | 12.56 | −1.10 | 258 | 16 | 14 |
| CH3NC | 11.78 | −1.13 | 11.92 | −1.16 | 258 | 16 | 14 |
| CH3F | 13.58 | −1.52 | 13.66 | −1.55 | 203 | 17 | 13 |
| CH2F2 | 13.73 | −1.53 | 13.76 | −1.56 | 235 | 17 | 13 |
| CHF3 | 15.16 | −1.55 | 15.25 | −1.58 | 267 | 17 | 13 |
| C2H6 | 12.99 | −1.53 | 12.90 | −1.56 | 284 | 15 | 13 |

TABLE XXXII. Ionization potentials and electron affinities at the $\omega$B97-X($+G3W2$)/QZ6P level of theory (in eV) as well as total number of molecular orbitals and size of imaginary time and imaginary frequency grids for the gw40 test set.

## B. Basis set limit extrapolated QP energies and comparison to EOM-CCSDT reference values

### 1. *qsGW - ionization potentials*

| molecule | CC | $GW$ | $GW+G3W2$ | $GW$ - CC | $GW+G3W2$ - CC |
|---|---|---|---|---|---|
| C2F4 | 10.70 | 10.85 | 10.66 | 0.15 | −0.04 |
| CF4 | 16.44 | 16.84 | 17.01 | 0.40 | 0.57 |
| SiF4 | 16.60 | 16.91 | 17.14 | 0.31 | 0.54 |
| HCN | 13.89 | 13.77 | 13.76 | −0.12 | −0.13 |
| C2H2 | 11.57 | 11.53 | 11.47 | −0.04 | −0.10 |
| HCCF | 11.53 | 11.53 | 11.43 | 0.00 | −0.10 |
| HCCCN | 11.86 | 12.02 | 11.92 | 0.16 | 0.06 |
| NNO | 13.01 | 12.88 | 12.91 | −0.13 | −0.10 |
| C2N2 | 13.66 | 13.60 | 13.56 | −0.06 | −0.10 |
| CO | 14.07 | 14.33 | 14.46 | 0.26 | 0.39 |
| CO2 | 13.92 | 14.09 | 14.21 | 0.17 | 0.29 |
| C3O2 | 10.86 | 11.17 | 11.09 | 0.31 | 0.23 |
| OCS | 11.35 | 11.47 | 11.44 | 0.12 | 0.09 |
| FCN | 13.73 | 13.82 | 13.78 | 0.09 | 0.05 |
| N2 | 15.68 | 16.04 | 16.23 | 0.36 | 0.55 |
| HC4H | 10.36 | 10.38 | 10.25 | 0.02 | −0.11 |
| HCl | 12.85 | 12.79 | 12.86 | −0.06 | 0.01 |
| HF | 16.32 | 16.59 | 16.87 | 0.27 | 0.55 |
| F2 | 15.91 | 16.58 | 16.79 | 0.67 | 0.88 |
| SiO | 11.54 | 11.67 | 11.74 | 0.13 | 0.20 |
| CS | 11.44 | 11.93 | 12.05 | 0.49 | 0.61 |
| P2 | 10.64 | 10.39 | 10.38 | −0.25 | −0.26 |
| H2CO | 11.01 | 11.29 | 11.31 | 0.28 | 0.30 |
| H2O | 12.82 | 12.85 | 13.09 | 0.03 | 0.27 |
| C2H4 | 10.78 | 10.70 | 10.61 | −0.08 | −0.17 |
| H2CS | 9.46 | 9.57 | 9.55 | 0.11 | 0.09 |
| HCONH2 | 10.49 | 10.84 | 10.94 | 0.35 | 0.45 |
| HCOOH | 11.64 | 11.81 | 11.90 | 0.17 | 0.26 |
| NSF | 11.96 | 12.20 | 12.26 | 0.24 | 0.30 |
| O3 | 12.89 | 13.37 | 13.60 | 0.48 | 0.71 |
| C2H2F2 | 10.77 | 10.86 | 10.73 | 0.09 | −0.04 |
| cisC2H2F2 | 10.67 | 10.74 | 10.61 | 0.07 | −0.06 |
| CH4 | 14.45 | 14.65 | 14.64 | 0.20 | 0.19 |
| CH3CCH | 10.61 | 10.67 | 10.57 | 0.06 | −0.04 |
| CH3CN | 12.62 | 12.67 | 12.62 | 0.05 | 0.00 |
| CH3NC | 11.39 | 11.92 | 12.05 | 0.53 | 0.66 |
| CH3F | 13.45 | 13.70 | 13.72 | 0.25 | 0.27 |
| CH2F2 | 13.58 | 13.92 | 13.89 | 0.34 | 0.31 |
| CHF3 | 15.07 | 15.40 | 15.41 | 0.33 | 0.34 |
| C2H6 | 12.77 | 13.06 | 12.96 | 0.29 | 0.19 |
| MADs = | | | | 0.21 | 0.27 |
| MDs = | | | | 0.18 | 0.20 |
| MAXs = | | | | 0.67 | 0.88 |
| r2 = | | | | 0.99 | 0.99 |

TABLE XXXIII. Ionization potentials for gw40: Experimental and EOM-CCSDT reference values and basis set limit extrapolated results for $GW$ and $GW+G3W2$ based on the qsGW starting point. The last three columns show deviations to the EOM-CCSDT reference values. Last for rows: Mean absolute deviations (MAD), mean signed deviations (MD), maximum errors (MAX), and Pearson correlation coefficients ($R^2$) All values are in eV.

*2. LRC-ωPBEh - ionization potentials*

| molecule | CC | $GW$ | $GW+G3W2$ | $GW$ - CC | $GW+G3W2$ - CC |
|---|---|---|---|---|---|
| C2F4 | 10.70 | 10.75 | 10.61 | 0.05 | −0.09 |
| CF4 | 16.44 | 16.55 | 16.93 | 0.11 | 0.49 |
| SiF4 | 16.60 | 16.63 | 17.30 | 0.03 | 0.70 |
| HCN | 13.89 | 13.79 | 13.78 | −0.10 | −0.11 |
| C2H2 | 11.57 | 11.50 | 11.41 | −0.07 | −0.16 |
| HCCF | 11.53 | 11.53 | 11.42 | 0.00 | −0.11 |
| HCCCN | 11.86 | 11.87 | 11.76 | 0.01 | −0.10 |
| NNO | 13.01 | 13.04 | 13.05 | 0.03 | 0.04 |
| C2N2 | 13.66 | 13.72 | 13.68 | 0.06 | 0.02 |
| CO | 14.07 | 14.23 | 14.35 | 0.16 | 0.28 |
| CO2 | 13.92 | 14.05 | 14.18 | 0.13 | 0.26 |
| C3O2 | 10.86 | 11.15 | 11.04 | 0.29 | 0.18 |
| OCS | 11.35 | 11.37 | 11.32 | 0.02 | −0.03 |
| FCN | 13.73 | 13.69 | 13.65 | −0.04 | −0.08 |
| N2 | 15.68 | 15.86 | 16.03 | 0.18 | 0.35 |
| HC4H | 10.36 | 10.38 | 10.21 | 0.02 | −0.15 |
| HCl | 12.85 | 12.74 | 12.82 | −0.11 | −0.03 |
| HF | 16.32 | 16.17 | 16.47 | −0.15 | 0.15 |
| F2 | 15.91 | 16.12 | 16.32 | 0.21 | 0.41 |
| SiO | 11.54 | 11.65 | 11.76 | 0.11 | 0.22 |
| CS | 11.44 | 11.70 | 11.83 | 0.26 | 0.39 |
| P2 | 10.64 | 10.39 | 10.36 | −0.25 | −0.28 |
| H2CO | 11.01 | 11.22 | 11.23 | 0.21 | 0.22 |
| H2O | 12.82 | 12.75 | 12.97 | −0.07 | 0.15 |
| C2H4 | 10.78 | 10.71 | 10.57 | −0.07 | −0.21 |
| H2CS | 9.46 | 9.53 | 9.49 | 0.07 | 0.03 |
| HCONH2 | 10.49 | 10.67 | 10.77 | 0.18 | 0.28 |
| HCOOH | 11.64 | 11.78 | 11.92 | 0.14 | 0.28 |
| NSF | 11.96 | 12.08 | 12.22 | 0.12 | 0.26 |
| O3 | 12.89 | 13.20 | 13.45 | 0.31 | 0.56 |
| C2H2F2 | 10.77 | 10.80 | 10.65 | 0.03 | −0.12 |
| cisC2H2F2 | 10.67 | 10.70 | 10.55 | 0.03 | −0.12 |
| CH4 | 14.45 | 14.60 | 14.59 | 0.15 | 0.14 |
| CH3CCH | 10.61 | 10.52 | 10.38 | −0.09 | −0.23 |
| CH3CN | 12.62 | 12.65 | 12.58 | 0.03 | −0.04 |
| CH3NC | 11.39 | 11.73 | 11.85 | 0.34 | 0.46 |
| CH3F | 13.45 | 13.64 | 13.67 | 0.19 | 0.22 |
| CH2F2 | 13.58 | 13.74 | 13.72 | 0.16 | 0.14 |
| CHF3 | 15.07 | 15.19 | 15.24 | 0.12 | 0.17 |
| C2H6 | 12.77 | 12.95 | 12.83 | 0.18 | 0.06 |
| MADs = | | | | 0.12 | 0.21 |
| MDs = | | | | 0.07 | 0.12 |
| MAXs = | | | | 0.34 | 0.70 |
| r2 = | | | | 1.00 | 0.99 |

TABLE XXXIV. Ionization potentials for gw40: Experimental and EOM-CCSDT reference values and basis set limit extrapolated results for $GW$ and $GW+G3W2$ based on the LRC-ωPBEh starting point. The last three columns show deviations to the EOM-CCSDT reference values. Last for rows: Mean absolute deviations (MAD), mean signed deviations (MD), maximum errors (MAX), and Pearson correlation coefficients ($R^2$) All values are in eV.

*3. ωB97-X - ionization potentials*

| molecule | CC | $GW$ | $GW+G3W2$ | $GW$ - CC | $GW+G3W2$ - CC |
|---|---|---|---|---|---|
| C2F4 | 10.70 | 10.86 | 10.72 | 0.16 | 0.02 |
| CF4 | 16.44 | 16.66 | 17.07 | 0.22 | 0.63 |
| SiF4 | 16.60 | 16.78 | 17.48 | 0.18 | 0.88 |
| HCN | 13.89 | 13.87 | 13.86 | −0.02 | −0.03 |
| C2H2 | 11.57 | 11.58 | 11.49 | 0.01 | −0.08 |
| HCCF | 11.53 | 11.59 | 11.48 | 0.06 | −0.05 |
| HCCCN | 11.86 | 11.96 | 11.84 | 0.10 | −0.02 |
| NNO | 13.01 | 13.12 | 13.14 | 0.11 | 0.13 |
| C2N2 | 13.66 | 13.75 | 13.70 | 0.09 | 0.04 |
| CO | 14.07 | 14.37 | 14.50 | 0.30 | 0.43 |
| CO2 | 13.92 | 14.11 | 14.25 | 0.19 | 0.33 |
| C3O2 | 10.86 | 11.19 | 11.09 | 0.33 | 0.23 |
| OCS | 11.35 | 11.44 | 11.40 | 0.09 | 0.05 |
| FCN | 13.73 | 13.79 | 13.75 | 0.06 | 0.02 |
| N2 | 15.68 | 16.06 | 16.24 | 0.38 | 0.56 |
| HC4H | 10.36 | 10.47 | 10.30 | 0.11 | −0.06 |
| HCl | 12.85 | 12.83 | 12.92 | −0.02 | 0.07 |
| HF | 16.32 | 16.28 | 16.60 | −0.04 | 0.28 |
| F2 | 15.91 | 16.24 | 16.47 | 0.33 | 0.56 |
| SiO | 11.54 | 11.74 | 11.85 | 0.20 | 0.31 |
| CS | 11.44 | 11.97 | 12.10 | 0.53 | 0.66 |
| P2 | 10.64 | 10.44 | 10.42 | −0.20 | −0.22 |
| H2CO | 11.01 | 11.32 | 11.33 | 0.31 | 0.32 |
| H2O | 12.82 | 12.79 | 13.03 | −0.03 | 0.21 |
| C2H4 | 10.78 | 10.79 | 10.67 | 0.01 | −0.11 |
| H2CS | 9.46 | 9.60 | 9.56 | 0.14 | 0.10 |
| HCONH2 | 10.49 | 10.80 | 10.90 | 0.31 | 0.41 |
| HCOOH | 11.64 | 11.90 | 12.05 | 0.26 | 0.41 |
| NSF | 11.96 | 12.16 | 12.29 | 0.20 | 0.33 |
| O3 | 12.89 | 13.60 | 13.88 | 0.71 | 0.99 |
| C2H2F2 | 10.77 | 11.07 | 10.93 | 0.30 | 0.16 |
| cisC2H2F2 | 10.67 | 10.81 | 10.66 | 0.14 | −0.01 |
| CH4 | 14.45 | 14.66 | 14.65 | 0.21 | 0.20 |
| CH3CCH | 10.61 | 10.77 | 10.63 | 0.16 | 0.02 |
| CH3CN | 12.62 | 12.71 | 12.64 | 0.09 | 0.02 |
| CH3NC | 11.39 | 11.91 | 12.05 | 0.52 | 0.66 |
| CH3F | 13.45 | 13.71 | 13.75 | 0.26 | 0.30 |
| CH2F2 | 13.58 | 13.86 | 13.85 | 0.28 | 0.27 |
| CHF3 | 15.07 | 15.30 | 15.36 | 0.23 | 0.29 |
| C2H6 | 12.77 | 13.07 | 12.94 | 0.30 | 0.17 |
| MADs = | | | | 0.20 | 0.27 |
| MDs = | | | | 0.19 | 0.24 |
| MAXs = | | | | 0.71 | 0.99 |
| r2 = | | | | 0.99 | 0.99 |

TABLE XXXV. Ionization potentials for gw40: Experimental and EOM-CCSDT reference values and basis set limit extrapolated results for $GW$ and $GW+G3W2$ based on the ωB97-X starting point. The last three columns show deviations to the EOM-CCSDT reference values. Last for rows: Mean absolute deviations (MAD), mean signed deviations (MD), maximum errors (MAX), and Pearson correlation coefficients ($R^2$) All values are in eV.

* a.t.l.foerster@vu.nl


[1] A. Förster and L. Visscher, J. Chem. Theory Comput. **17**, 5080 (2021).
[2] S. J. Chakravorty, S. R. Gwaltney, E. R. Davidson, F. A. Parpia, and C. F. Fischer, Phys. Rev. A **47**, 3649 (1993).
[3] S. P. McCarthy and A. J. Thakkar, J. Chem. Phys. **134** (2011), 10.1063/1.3547262.
